# Supplementary material for: Online Inference with Multi-modal Likelihood Functions
Source: arXiv:1809.11108 source file (2020-10-19)
Supplement: Supplementary file 1 [file supplement.pdf]

# Supplementary materials for "Perturbed Bayesian Inference for Online Parameter Estimation"

Mathieu Gerber* Kari Heine†

Unless otherwise state, the notation used below refers to the objects defined in Algorithm 1 and in Conditions C1-C4 of Section 2.3. Let $\sigma(X)$ the $\sigma$-algebra generated by random variable $X$ and $\mathbb{N}_0 = \{0\} \cup \mathbb{N}$.

## S1 Preliminary results

### S1.1 A technical lemma

The following result seems to be common knowledge but its original proof is difficult track back.

**Lemma S1.** *Let $A \in \mathcal{F}$ be such that $\mathbb{P}(A) > 0$. Then,*

$$\sup_{B\in\mathcal{F}} \big|\mathbb{P}(B|A) - \mathbb{P}(B)\big| = 1 - \mathbb{P}(A).$$

*Proof.* Let $B \in \mathcal{F}$ and note that $\mathbb{P}(B|A) - \mathbb{P}(B) = b(1-a)/a - c$ where

$$a = \mathbb{P}(A), \quad b = \mathbb{P}(B \cap A), \quad c = \mathbb{P}(B \setminus A).$$

Then, because $0 \le b \le a$ and $0 \le c \le 1-a$, we have

$$-(1-a) \le -c \le \mathbb{P}(B|A) - \mathbb{P}(B) \le b(1-a)/a \le 1-a$$

and thus

$$\sup_{B\in\mathcal{F}} \big|\mathbb{P}(B|A) - \mathbb{P}(B)\big| = 1 - a = 1 - \mathbb{P}(A).$$

□

*School of Mathematics, University of Bristol, UK.
†Department of Mathematical Sciences, University of Bath, UK.

## S1.2 Two preliminary lemmas

**Lemma S2.** *Assume A1-A5, let* $(\tilde{c}_j)_{j\geq 0}$ *be a sequence in* $(0,1]$ *and, for every* $(p,j)\in\mathbb{N}_0^2$*, let* $\tilde{\epsilon}_{p,j}=\tilde{c}_j\epsilon_p$ *and* $\tau_{p,j+1}=t_{p+j+1}-t_{p+j}$*.*

*Let*

$$K_\kappa=\inf\big\{k\in\mathbb{N}:\,k>\kappa^{-1}L_\star\big\},\quad L_\star=D^{-1/2}\big(\mathbb{E}[m_{\theta_\star}^2]\vee d\|V_{\theta_\star}\|\big)^{1/2} \tag{S.1}$$

*with,* $m_{\theta_\star}$ *as in A3,* $V_{\theta_\star}$ *as in Lemma S11 and* $D\in\mathbb{R}_{>0}$ *as in Lemma S13. Let* $\lambda>0$ *and* $\bar{\alpha}>0$ *be such that*

$$K_\kappa\geq\kappa^{-1}L_\star(1+\bar{\alpha})^{1/2}(1+\lambda)^{1/2}. \tag{S.2}$$

*Then, for every* $\alpha\in(0,\bar{\alpha})$ *and* $\underline{c}\in(0,1)$*, there exists a constant* $\bar{c}\in\mathbb{R}_{>0}$ *such that, for every* $(p,j)\in\mathbb{N}^2$ *and* $\eta\in\mathcal{P}(\Theta)$ *with* $\eta\big(B_{\tilde{\epsilon}_{p,j-1}/K_\kappa}(\theta_\star)\big)\geq\underline{c}$*, we have*

$$\mathbb{E}\big[\Psi_{t_{p+j-1}:t_{p+j}}(\eta)\big(B^c_{\kappa_\alpha\tilde{\epsilon}_{p,j-1}}(\theta_\star)\big)\,|\,\sigma\big(Y_{1:t_{p+j-1}}\big)\big]\leq\bar{c}\Big(\tau_{p,j}^{-1/2}+\tau_{p,j}^{-1}\tilde{\epsilon}_{p,j-1}^{-2}\Big),\quad\mathbb{P}-a.s.$$

*where* $\kappa_\alpha=\kappa\sqrt{(1+\alpha)/(1+\bar{\alpha})}$*.*

See Section S6.2 for a proof.

**Corollary 1.** *Let* $L_\star$ *be as defined in* (S.1)*. Then,* $L_\star>1$*.*

*Proof.* Let $K_\kappa$ be as defined in (S.1) and assume that $L_\star\in(0,1)$. In this case, there exists e $\lambda>0$ and $\bar{\alpha}>0$ such that (S.2) holds and such that, for some $\alpha\in(0,\bar{\alpha})$,

$$K_\kappa^{-1}>\kappa_\alpha=\kappa\sqrt{\frac{1+\alpha}{1+\bar{\alpha}}}\geq\frac{\kappa}{\sqrt{(1+\bar{\alpha})(1+\lambda)}}.$$

Then, it is easily checked that there exists probability measure $\eta'\in\mathcal{P}(\Theta)$ such that $\eta'\big(B_{\tilde{\epsilon}_{p,j-1}/K_\kappa}(\theta_\star)\big)\geq\underline{c}$ and such that $\eta'\big(B^c_{\kappa_\alpha\tilde{\epsilon}_{p,j-1}}(\theta_\star)\big)=1$. Consequently, we have $\Psi_{t_{p+j-1}:t_{p+j}}(\eta')\big(B^c_{\kappa_\alpha\tilde{\epsilon}_{p,j-1}}(\theta_\star)\big)=1$, $\mathbb{P}$-almost surely, which contradicts the conclusion of Lemma S2. The result follows. □

**Lemma S3.** *Assume A1-A2, A5-A7 and C2, and let* $(\tilde{\epsilon}_p)_{p\geq 0}$ *be a sequence in* $\mathbb{R}_{>0}$ *verifying* $\lim_{p\to+\infty}(t_p-t_{p-1})^{1/2}\tilde{\epsilon}_p=+\infty$ *and* $\lim_{p\to+\infty}\tilde{\epsilon}_p=0$*. Then, there exist*

- *constants* $\underline{p}\in\mathbb{N}$, $\underline{c}\in\mathbb{R}_{>0}$ *and* $c_\star\in(0,1)$
- *a sequence* $(\Omega_{p,\tilde{\epsilon}_p})_{p\geq 1}$ *in* $\mathcal{F}$ *such that* $\lim_{p\to+\infty}\mathbb{P}(\Omega_{p,\tilde{\epsilon}_p})=1$ *and such that for all* $p\geq 1$ *the random set* $\Omega_{p,\tilde{\epsilon}_p}$ *is* $\sigma(Y_{(t_{p-1}+1):t_p})$ *measurable,*

*such that,* $\mathbb{P}$*-a.s., we have for all* $M\geq 1$*,* $N\geq 1$ *and* $p\geq\underline{p}$*,*

$$\begin{aligned}\mathbb{P}\big(\bar{\vartheta}_{t_p}^{(2)}\in &B_{\tilde{\epsilon}_p}(\theta_\star)|\,\Omega_{p,\tilde{\epsilon}_p},\,\sigma\big(Y_{1:t_p},\vartheta^{1:\tilde{N}}_{t_0:t_{p-2}},\theta^{1:N}_{t_0:t_{p-1}}\big)\big)\\ &\geq\mathbb{P}\big(\exists n\in 1:M\text{ s.t. }\vartheta^{N+n}_{t_{p-1}}\in B_{c_\star\tilde{\epsilon}_p}(\theta_\star)\,|\,\Omega_{p,\tilde{\epsilon}_p},\,\sigma\big(Y_{1:t_p},\vartheta^{1:\tilde{N}}_{t_0:t_{p-2}},\theta^{1:N}_{t_0:t_{p-1}}\big)\big)\\ &\geq\underline{c}\,\gamma^\nu_{t_{p-1}}\tilde{\epsilon}_p^d\end{aligned}$$

*where* $\bar{\vartheta}^{(2)}_{t_p}=\vartheta^{n_p}_{t_{p-1}}$ *with* $n_p\in\operatorname{argmax}_{1:\tilde{N}}\tilde{w}^n_{t_p}$*.*

See Section S6.3 for a proof.

## S1.3 Preliminary results for the auxiliary sequence of PPDs

### S1.3.1 Under Conditions C2 and C4

**Lemma S4.** *Assume A1-A5, C2 and C4. Then, there exists a constant $\bar{c}\in\mathbb{R}_{>0}$ such that*

$$\sup_{(M,N)\in\mathcal{Q}_\kappa}\mathbb{P}\big(\bar{\vartheta}_{t_p}\not\in B_{\epsilon_p}(\theta_\star)|\,\bar{\vartheta}_{t_{p-1}}\in B_{\epsilon_{p-1}}(\theta_\star)\big)\leq \bar{c}\,(t_p-t_{p-1})^{-1/2},\quad \forall p\in\mathbb{N}$$

*where $\mathcal{Q}_\kappa=\{(M,N)\in\mathbb{N}^2:\ N\geq(2K_\kappa)^d\}$, with $K_\kappa$ defined in* (S.1).

*Proof.* Let $(M,N)\in\mathcal{Q}_\kappa$. Below $\underline{p}\in\mathbb{N}$ is a constant (independent of $N$ and $M$) whose value can change from one expression to another.

For every $p\in\mathbb{N}$ let $\tau_p=t_p-t_{p-1}$. Let $\lambda>0$ and $\bar{\alpha}>0$ be such that (S.2) holds, $\underline{\kappa}=\kappa\sqrt{(1+\bar{\alpha}/2)/(1+\bar{\alpha})}$ and $v:[0,1]\to\mathbb{R}_{>0}$ be such that

$$\mathbb{E}\big[\Psi_{t_{p-1}:t_p}(\eta)\big(B^c_{\underline{\kappa}\epsilon_p}(\theta_\star)\big)\big]\leq v(c)\,\tau_p^{-1/2}\tag{S.3}$$

for every $p\geq 1$ and $\eta\in\mathcal{P}(\Theta)$ verifying $\eta\big(B_{\epsilon_{p-1}/K_\kappa}(\theta_\star)\big)\geq c$. Note that under A1-A5 such a mapping $v:[0,1]\to\mathbb{R}_{>0}$ exists by Lemma S2 (with $\tilde{c}_1=1$ and $j=1$) and because $\tau_p^{-1}\epsilon_{p-1}^2\leq\bar{c}\,\tau_p^{-1}$ for all $p\geq 1$ and some constant $\bar{c}<+\infty$.

For every $p\in\mathbb{N}$ let $\bar{\vartheta}^{(2)}_{t_p}$ be as in Lemma S3 and

$$J_{p-1}=\big\{n\in 1:M\text{ s.t. }\vartheta^{N+n}_{t_{p-1}}\in B_{(1+2\kappa)\epsilon_{p-1}}(\bar{\vartheta}_{t_{p-1}})\big\},\quad \tilde{J}_{p-1}=1:N\cup J_{p-1}\tag{S.4}$$

$$\bar{\vartheta}^{(1)}_{t_p}=\sum_{n\in\tilde{J}_{p-1}}\widehat{W}^n_{t_p}\vartheta^n_{t_{p-1}},\quad Z_p=\sum_{n=1}^{\tilde{N}}\frac{a_n\tilde{w}^n_{t_p}}{\sum_{m=1}^{\tilde{N}}a_m\tilde{w}^m_{t_p}}\mathbb{1}\big(\vartheta^n_{t_{p-1}}\in B_{(1+\kappa)\epsilon_{p-1}}(\bar{\vartheta}_{t_{p-1}})\big)\tag{S.5}$$

and

$$\widehat{W}^n_{t_p}=\frac{\hat{w}^n_{t_p}\hat{a}_n(J_{p-1})}{\sum_{m\in\tilde{J}_{p-1}}\hat{w}^m_{t_p}\hat{a}_m(J_{p-1})},\ n\in\tilde{J}_{p-1}$$

where $a_{1:\tilde{N}}$ and $\hat{a}_{1:\tilde{N}}(J)$ are as in C4, for $J\subset(N+1):\tilde{N}$.

Then, under C4 and for every $p\geq 1$,

$$\begin{aligned}\mathbb{P}\big(\bar{\vartheta}_{t_p}\not\in B_{\epsilon_p}(\theta_\star)|\,\bar{\vartheta}_{t_{p-1}}\in B_{\epsilon_{p-1}}(\theta_\star)\big)&\\ &=\mathbb{P}\big(\bar{\vartheta}^{(1)}_{t_p}\not\in B_{\epsilon_p}(\theta_\star),Z_p>\Delta|\,\bar{\vartheta}_{t_{p-1}}\in B_{\epsilon_{p-1}}(\theta_\star)\big)\\ &+\mathbb{P}\big(\bar{\vartheta}^{(2)}_{t_p}\not\in B_{\epsilon_p}(\theta_\star),\,Z_p\leq\Delta|\,\bar{\vartheta}_{t_{p-1}}\in B_{\epsilon_{p-1}}(\theta_\star)\big)\\ &\leq\mathbb{P}\big(\bar{\vartheta}^{(1)}_{t_p}\not\in B_{\epsilon_p}(\theta_\star)|\,\bar{\vartheta}_{t_{p-1}}\in B_{\epsilon_{p-1}}(\theta_\star)\big)\\ &+\mathbb{P}\big(Z_p\leq\Delta|\,\bar{\vartheta}_{t_{p-1}}\in B_{\epsilon_{p-1}}(\theta_\star)\big).\end{aligned}\tag{S.6}$$

In the remainder of the proof we find upper bounds for the two terms appearing on the r.h.s. of (S.6).

For every $p \geq 1$ let

$$\mu_{p-1} = \sum_{n=1}^{\tilde{N}} \frac{a_n}{(1+\zeta_1)M - (1-\zeta_2)} \, \delta_{\vartheta^n_{t_{p-1}}}. \tag{S.7}$$

Note that $\mu_{p-1}$ is a random probability measure on $\Theta$.

Then, for the second term on the r.h.s. of (S.6) we have, for all $p \geq 1$,

$$\begin{aligned}&\mathbb{P}\big(Z_p \leq \Delta \big|\, \bar{\vartheta}_{t_{p-1}} \in B_{\epsilon_{p-1}}(\theta_\star)\big)\\ &\qquad \leq \mathbb{P}\Big(\Psi_{t_{p-1}:t_p}(\mu_{p-1})\big(B^c_{\kappa\epsilon_{p-1}}(\theta_\star)\big) \geq 1-\Delta \big|\, \bar{\vartheta}_{t_{p-1}} \in B_{\epsilon_{p-1}}(\theta_\star)\Big).\end{aligned}$$

Since $N \geq (2K_\kappa)^d$ we have, under C2 and for some constant $\tilde{c} > 0$,

$$\mathbb{P}\big(\bar{\vartheta}_{t_{p-1}} \in B_{\epsilon_{p-1}}(\theta_\star)\big) = \mathbb{P}\Big(\bar{\vartheta}_{t_{p-1}} \in B_{\epsilon_{p-1}}(\theta_\star),\, \mu_{p-1}\big(B_{\epsilon_{p-1}/K_\kappa}(\theta_\star)\big) \geq \frac{\zeta_1}{1+\zeta_1} \tilde{c}\, K_\kappa^{-d}\Big)$$

and thus, under A2, C2 and C4, and using (S.3) and Markov's inequality, we have for all $p \geq 1$,

$$\mathbb{P}\big(Z_p \leq \Delta \big|\, \bar{\vartheta}_{t_{p-1}} \in B_{\epsilon_{p-1}}(\theta_\star)\big) \leq \frac{v\big(\zeta_1\, \tilde{c}\, K_\kappa^{-d}/(1+\zeta_1)\big)}{1-\Delta}\, \tau_p^{-1/2}. \tag{S.8}$$

To find an upper bound the second term in (S.6) we define for every $p \geq 1$,

$$\hat{\mu}_{p-1} = \sum_{n \in \tilde{J}_{p-1}} \widehat{W}^n_{t_p}\, \delta_{\vartheta^n_{t_{p-1}}}. \tag{S.9}$$

Note that $\hat{\mu}_{p-1}$ is a random probability measure on $\Theta$.

Then, for all $p \geq 1$ we have

$$\begin{aligned}&\mathbb{P}\Big(\bar{\vartheta}^{(1)}_{t_p} \notin B_{\epsilon_p}(\theta_\star) \big|\, \bar{\vartheta}_{t_{p-1}} \in B_{\epsilon_{p-1}}(\theta_\star)\Big)\\ &= \mathbb{P}\Big(\Big\| \sum_{n \in \tilde{J}_{p-1}} \widehat{W}^n_{t_p}(\vartheta^n_{t_{p-1}} - \theta_\star)\mathbb{1}\big(\vartheta^n_{t_{p-1}} \in B_{\underline{\kappa}\epsilon_{p-1}}(\theta_\star)\big)\\ &\qquad + \sum_{n \in \tilde{J}_{p-1}} \widehat{W}^n_{t_p}(\vartheta^n_{t_{p-1}} - \theta_\star)\mathbb{1}\big(\vartheta^n_{t_{p-1}} \notin B_{\underline{\kappa}\epsilon_{p-1}}(\theta_\star)\big)\Big\| \geq \epsilon_p \big|\, \bar{\vartheta}_{t_{p-1}} \in B_{\epsilon_{p-1}}(\theta_\star)\Big) \qquad \text{(S.10)}\\ &\leq \mathbb{P}\Big(\underline{\kappa}\epsilon_{p-1} + 2(1+\kappa)\epsilon_{p-1}\Psi_{t_{p-1}:t_p}(\hat{\mu}_{p-1})\big(B^c_{\underline{\kappa}\epsilon_{p-1}}(\theta_\star)\big) \geq \epsilon_p \big|\, \bar{\vartheta}_{t_{p-1}} \in B_{\epsilon_{p-1}}(\theta_\star)\Big)\\ &= \mathbb{P}\Big(\Psi_{t_{p-1}:t_p}(\hat{\mu}_{p-1})\big(B^c_{\underline{\kappa}\epsilon_{p-1}}(\theta_\star)\big) \geq \frac{\epsilon_p - \underline{\kappa}\epsilon_{p-1}}{2(1+\kappa)\epsilon_{p-1}} \big|\, \bar{\vartheta}_{t_{p-1}} \in B_{\epsilon_{p-1}}(\theta_\star)\Big).\end{aligned}$$

To proceed further not that $(\epsilon_p)_{p\geq 1}$ is such that $\epsilon_p \geq \kappa\epsilon_{p-1}$ for all $r \geq \underline{p}$, and therefore, for very $p \geq \underline{p}$ we have

$$\begin{aligned}&\mathbb{P}\Big(\bar{\vartheta}^{(1)}_{t_p} \notin B_{\epsilon_p}(\theta_\star) \big|\, \bar{\vartheta}_{t_{p-1}} \in B_{\epsilon_{p-1}}(\theta_\star)\Big)\\ &\qquad \leq \mathbb{P}\Big(\Psi_{t_{p-1}:t_p}(\hat{\mu}_{p-1})\big(B^c_{\underline{\kappa}\epsilon_{p-1}}(\theta_\star)\big) \geq \frac{\kappa\epsilon_{p-1} - \underline{\kappa}\epsilon_{p-1}}{2(1+\kappa)\epsilon_{p-1}} \big|\, \bar{\vartheta}_{t_{p-1}} \in B_{\epsilon_{p-1}}(\theta_\star)\Big) \qquad \text{(S.11)}\\ &\qquad = \mathbb{P}\Big(\Psi_{t_{p-1}:t_p}(\hat{\mu}_{p-1})\big(B^c_{\underline{\kappa}\epsilon_{p-1}}(\theta_\star)\big) \geq c_\kappa \big|\, \bar{\vartheta}_{t_{p-1}} \in B_{\epsilon_{p-1}}(\theta_\star)\Big)\end{aligned}$$

with $c_\kappa = \frac{\kappa-\underline{\kappa}}{2(1+\kappa)} > 0$.

Since $N \geq (2K_\kappa)^d$ we have, under C2,

$$\mathbb{P}\big(\bar{\vartheta}_{t_{p-1}} \in B_{\epsilon_{p-1}}(\theta_\star)\big) = \mathbb{P}\Big(\bar{\vartheta}_{t_{p-1}} \in B_{\epsilon_{p-1}}(\theta_\star),\, \hat{\mu}_{p-1}\big(B_{\epsilon_{p-1}/K_\kappa}(\theta_\star)\big) \geq \frac{\zeta_3}{1+\zeta_3}\tilde{c}K_\kappa^{-d}\Big\}$$

with $\tilde{c} > 0$ as per above. Therefore, under A2, C2 and C4, and using (S.3) and Markov's inequality, this shows that, for any $p \geq \underline{p}$,

$$\begin{aligned}
&\mathbb{P}\big(\bar{\vartheta}_{t_p}^{(1)} \not\in B_{\epsilon_p}(\theta_\star) |\, \hat{\vartheta}_{t_{p-1}} \in B_{\epsilon_{p-1}}(\theta_\star)\big)\\
&\qquad \leq \mathbb{P}\Big(\Psi_{t_{p-1}:t_p}(\hat{\mu}_{p-1})\big(B^c_{\underline{\kappa}\epsilon_{p-1}}(\theta_\star)\big) \geq c_\kappa |\, \hat{\vartheta}_{t_{p-1}} \in B_{\epsilon_{p-1}}(\theta_\star)\Big)\\
&\qquad \leq \frac{v\big(\zeta_3\, \tilde{c}\, K_\kappa^{-d}/(1+\zeta_3)\big)}{c_\kappa}\, \tau_p^{-1/2}.
\end{aligned}$$

Together with (S.6) and (S.8), this completes the proof. □

**Lemma S5.** *Assume A1-A7, C2 and C4. Then, there exist constants* $\underline{c} \in \mathbb{R}_{>0}$ *and* $\bar{p} \in \mathbb{N}$ *such that*

$$\sup_{(N,M)\in\mathcal{Q}_\kappa} \mathbb{P}\big(\bar{\vartheta}_{t_p} \not\in B_{\epsilon_p}(\theta_\star) |\, \bar{\vartheta}_{t_{p-1}} \not\in B_{\epsilon_{p-1}}(\theta_\star)\big) \leq 1 - \underline{c}\,\gamma^\nu_{t_{p-1}}\epsilon^d_{p-1}, \quad \forall p \geq \underline{p}$$

*with* $\mathcal{Q}_\kappa$ *as in Lemma S4.*

*Proof.* Let $(M,N) \in \mathcal{Q}_\kappa$. Below, $\underline{c} \in \mathbb{R}_{>0}$ and $\underline{p} \in \mathbb{N}$ are two constants (independent of $N$ and $M$) whose values can change from one expression to another.

Let $c_\star > 0$ be as in the statement of Lemma S3 and, for $p \geq 1$, let $\tilde{\epsilon}_p = c_\star \epsilon_{p-1}$ and $\Omega_{p,\tilde{\epsilon}_p}$ be as in the statement of Lemma S3. Without loss of generality, we assume below that $c_* \leq \min(\kappa/2, k^{-1}_{\kappa/2})$ (with $k_{\kappa/2}$ defined in (S.1)).

Then, under A2, C2 and C4, we have for every $p \geq 1$

$$\begin{aligned}
&\mathbb{P}\big(\bar{\vartheta}_{t_p} \not\in B_{\epsilon_p}(\theta_\star) |\, \bar{\vartheta}_{t_{p-1}} \not\in B_{\epsilon_{p-1}}(\theta_\star)\big)\\
&\qquad = 1 - \mathbb{P}\big(\bar{\vartheta}_{t_p} \in B_{\epsilon_p}(\theta_\star) |\, \hat{\vartheta}_{t_{r-1}} \not\in B_{\epsilon_{p-1}}(\theta_\star)\big)\\
&\qquad \leq 1 - \mathbb{P}\big(\bar{\vartheta}_{t_p} \in B_{\epsilon_p}(\theta_\star) |\, \bar{\vartheta}_{t_{p-1}} \not\in B_{\epsilon_{p-1}}(\theta_\star),\, \Omega_{p,\tilde{\epsilon}_p}\big)\mathbb{P}(\Omega_{p,\tilde{\epsilon}_p})
\end{aligned} \tag{S.12}$$

where, under C4,

$$\begin{aligned}
&\mathbb{P}\big(\bar{\vartheta}_{t_p} \in B_{\epsilon_p}(\theta_\star) |\, \bar{\vartheta}_{t_{p-1}} \not\in B_{\epsilon_{p-1}}(\theta_\star),\, \Omega_{p,\tilde{\epsilon}_p}\big)\\
&\qquad = \mathbb{P}\big(\bar{\vartheta}^{(1)}_{t_p} \in B_{\epsilon_p}(\theta_\star),\, Z_p > \Delta |\, \hat{\vartheta}_{t_{p-1}} \not\in B_{\epsilon_{p-1}}(\theta_\star),\, \Omega_{p,\tilde{\epsilon}_p}\big)\\
&\qquad + \mathbb{P}\big(\bar{\vartheta}^{(2)}_{t_p} \in B_{\epsilon_p}(\theta_\star),\, Z_p \leq \Delta |\, \bar{\vartheta}_{t_{p-1}} \not\in B_{\epsilon_{p-1}}(\theta_\star),\, \Omega_{p,\tilde{\epsilon}_p}\big)
\end{aligned} \tag{S.13}$$

with $Z_p$ and $\bar{\vartheta}^{(1)}_{t_p}$ defined in (S.5) and $\bar{\vartheta}^{(2)}_{t_p}$ defined in the statement of Lemma S3. We now find lower bounds for the two terms on the r.h.s. of (S.13).

For every $p \geq 1$ let $\Omega'_{p-1} = \big\{\vartheta^{N+1}_{t_{p-1}} \in B_{c_\star \epsilon_{p-1}}(\theta_\star),\, \bar{\vartheta}_{t_{p-1}} \notin B_{\epsilon_{p-1}}(\theta_\star)\big\}$ and

$$b_p = \mathbb{P}\big(Z_p \leq \Delta |\, \Omega'_{p-1},\, \Omega_{p,\epsilon_p}\big).$$

Then, for the second probability appearing on r.h.s. of (S.13) we have, for all $p \geq 1$,

$$\begin{aligned} &\mathbb{P}\big(\bar{\vartheta}^{(2)}_{t_p} \in B_{\epsilon_p}(\theta_\star),\, Z_p \leq \Delta |\, \bar{\vartheta}_{t_{p-1}} \notin B_{\epsilon_{p-1}}(\theta_\star),\, \Omega_{p,\tilde{\epsilon}_p}\big) \\ &\qquad \geq b_p\, \mathbb{P}\big(\bar{\vartheta}^{(2)}_{t_p} \in B_{\epsilon_p}(\theta_\star) |\, Z_p \leq \Delta,\, \Omega'_{p-1},\, \Omega_{p,\tilde{\epsilon}_p}\big) \\ &\qquad \times \mathbb{P}\big(\vartheta^{N+1}_{t_{p-1}} \in B_{c_\star \epsilon_{p-1}}(\theta_\star) |\, \bar{\vartheta}_{t_{p-1}} \notin B_{\epsilon_{p-1}}(\theta_\star),\, \Omega_{p,\tilde{\epsilon}_p}\big) \end{aligned} \tag{S.14}$$

where, by Lemma S3, for all $p \geq \underline{p}$ we have both

$$\mathbb{P}\big(\vartheta^{N+1}_{t_{p-1}} \in B_{c_\star \epsilon_{p-1}}(\theta_\star) |\, \bar{\vartheta}_{t_{p-1}} \notin B_{\epsilon_{p-1}}(\theta_\star),\, \Omega_{p,\tilde{\epsilon}_p}\big) \geq \underline{c}\, \gamma^{\nu}_{t_{p-1}} \epsilon^d_{p-1} \tag{S.15}$$

and (with $\underline{p}$ is such that $\epsilon_p \geq \kappa \epsilon_{p-1} \geq \tilde{\epsilon}_p$)

$$\mathbb{P}\big(\bar{\vartheta}^{(2)}_{t_p} \in B_{\epsilon_p}(\theta_\star) |\, Z_p \leq \Delta,\, \Omega'_{p-1},\, \Omega_{p,\tilde{\epsilon}_p}\big) = 1. \tag{S.16}$$

Then, combining (S.14)-(S.16) yields

$$\mathbb{P}\big(\bar{\vartheta}^{(2)}_{t_p} \in B_{\epsilon_p}(\theta_\star),\, Z_p \leq \Delta |\, \bar{\vartheta}_{t_{p-1}} \notin B_{\epsilon_{p-1}}(\theta_\star),\, \Omega_{p,\tilde{\epsilon}_p}\big) \geq b_p\, \underline{c}\, \gamma^{\nu}_{t_{p-1}} \epsilon^d_{p-1}, \quad \forall p \geq \underline{p}. \tag{S.17}$$

Next, for the first probability appearing on the r.h.s. of (S.13), we have

$$\begin{aligned} &\mathbb{P}\big(\bar{\vartheta}^{(1)}_{t_p} \in B_{\epsilon_p}(\theta_\star),\, Z_p > \Delta |\, \bar{\vartheta}_{t_{p-1}} \notin B_{\epsilon_{p-1}}(\theta_\star),\, \Omega_{p,\tilde{\epsilon}_p}\big) \\ &\qquad \geq (1 - b_p) \mathbb{P}\big(\bar{\vartheta}^{(1)}_{t_p} \in B_{\epsilon_p}(\theta_\star) |\, Z_p > \Delta,\, \Omega'_{p-1},\, \Omega_{p,\tilde{\epsilon}_p}\big) \\ &\qquad \times \mathbb{P}\big(\vartheta^{N+1}_{t_{p-1}} \in B_{c_\star \epsilon_{p-1}}(\theta_\star) |\, \bar{\vartheta}_{t_{p-1}} \notin B_{\epsilon_{p-1}}(\theta_\star),\, \Omega_{p,\tilde{\epsilon}_p}\big) \\ &\qquad \geq (1 - b_p) \mathbb{P}\big(\bar{\vartheta}^{(1)}_{t_p} \in B_{\epsilon_p}(\theta_\star) |\, Z_p > \Delta,\, \Omega'_{p-1},\, \Omega_{p,\tilde{\epsilon}_p}\big)\, \underline{c}\, \gamma^{\nu}_{t_{p-1}} \epsilon^d_{p-1} \end{aligned} \tag{S.18}$$

where the last inequality uses (S.15) and holds for $p \geq \underline{p}$. We now find a lower bound for the second term on the r.h.s. of (S.18).

Let $\delta \in (0, 1)$ be such that $\delta + \Delta > 1$ (note that such a $\delta$ exists because $\Delta > 0$ under C4) and, for every $p \geq 1$, let $\tilde{\Psi}_p = \Psi_{t_{p-1}:t_p}(\mu_{p-1})\big(B_{\kappa \epsilon_{p-1}/2}(\theta_\star)\big)$ with $\mu_{p-1}$ defined in (S.7). Then,

$$\mathbb{P}\big(\bar{\vartheta}^{(1)}_{t_p} \in B_{\epsilon_p}(\theta_\star) |\, Z_p > \Delta,\, \Omega'_{p-1},\, \Omega_{p,\tilde{\epsilon}_p}\big) \geq b_{p,1}\, b_{p,2} \tag{S.19}$$

where

$$\begin{aligned} &b_{p,1} := \mathbb{P}\big(\bar{\vartheta}^{(1)}_{t_p} \in B_{\epsilon_p}(\theta_\star) \,|\, \tilde{\Psi}_p > \delta,\, Z_p > \Delta,\, \Omega'_{p-1},\, \Omega_{p,\tilde{\epsilon}_p}\big) \\ &b_{p,2} = \mathbb{P}\big(\tilde{\Psi}_p > \delta |\, Z_p > \Delta,\, \Omega'_{p-1},\, \Omega_{p,\tilde{\epsilon}_p}\big) \end{aligned}$$

and we now show that for every $(c_1,c_2)\in(0,1)^2$ there exists a $p_{c_1,c_2}\in\mathbb{N}$ (independent of $N$ and $M$) such that

$$b_{p,1}\geq(1-b_p)-c_1,\quad b_{p,2}\geq c_2-b_p,\quad \forall p\geq p_{c_1,c_2}. \tag{S.20}$$

We start by studying $b_{p,1}$. Because $\Delta+\delta>1$, for all $p\geq 1$ we have

$$\begin{aligned}
&\big\{\tilde\Psi_p>\delta,\, Z_p>\Delta,\, \Omega'_{p-1},\, \Omega_{p,\tilde\epsilon_p}\big\}\\
&=\big\{\tilde\Psi_p>\delta,\, Z_p>\Delta,\, B_{\kappa\epsilon_{p-1}/2}(\theta_\star)\cap B_{(1+\kappa)\epsilon_{p-1}}(\bar\vartheta_{t_{p-1}})\neq\varnothing,\, \Omega'_{p-1},\, \Omega_{p,\tilde\epsilon_p}\big\}\\
&=\big\{\tilde\Psi_p>\delta,\; Z_p>\Delta,\, \bar\vartheta_{t_{p-1}}\in B_{(2+3\kappa)\epsilon_{p-1}/2}(\theta_\star),\, \Omega'_{p-1},\, \Omega_{p,\tilde\epsilon_p}\big\}\\
&=\big\{\tilde\Psi_p>\delta,\, Z_p>\Delta,\, \bar\vartheta_{t_{p-1}}\in B_{(2+3\kappa)\epsilon_{p-1}/2}(\theta_\star),\, N+1\in\tilde J_{p-1},\, \Omega'_{p-1},\, \Omega_{p,\tilde\epsilon_p}\big\}
\end{aligned} \tag{S.21}$$

where the last equality uses the fact that, in the definition of $\Omega'_{p-1}$, $c_*<\kappa/2$ and where $\tilde J_{p-1}$ is defined in (S.4).

For every $p\geq 1$ let $\tilde\Omega_{p-1}=\big\{\bar\vartheta_{t_{p-1}}\in B_{(2+3\kappa)\epsilon_{p-1}/2}(\theta_\star),\, N+1\in\tilde J_{p-1}\big\}$ and, with $\hat\mu_{p-1}$ as in (S.9), let $\hat\Psi_p=\Psi_{t_{p-1}:t_p}(\hat\mu_{p-1})\big(B_{\kappa\epsilon_{p-1}/2}(\theta_\star)\big)$.

Let $c'_\kappa=\frac{\kappa}{4+7\kappa}$. Then, for all $p\geq\underline{p}$, we have

$$\begin{aligned}
&\mathbb{P}\big(\bar\vartheta^{(1)}_{t_p}\notin B_{\epsilon_p}(\theta_\star)\big|\,\tilde\Psi_p>\delta,\, Z_p>\Delta,\, \Omega'_{p-1},\, \Omega_{p,\tilde\epsilon_p}\big)\\
&\quad=\mathbb{P}\big(\bar\vartheta^{(1)}_{t_p}\notin B_{\epsilon_p}(\theta_\star)\big|\,\tilde\Psi_p>\delta,\, Z_p>\Delta,\, \tilde\Omega_{p-1},\, \Omega'_{p-1},\, \Omega_{p,\tilde\epsilon_p}\big)\\
&\quad\leq\mathbb{P}\big(1-\hat\Psi_p\geq c'_\kappa\big|\,\tilde\Psi_p>\delta,\, Z_p>\Delta,\, \tilde\Omega_{p-1},\, \Omega'_{p-1},\, \Omega_{p,\tilde\epsilon_p}\big)
\end{aligned} \tag{S.22}$$

where the equality uses (S.21) and the inequality follows from similar computations as in (S.10) and (S.11).

Therefore, using (S.22), for all $p\geq\underline{p}$

$$\begin{aligned}
b_{p,1}&\geq\mathbb{P}\big(\hat\Psi_p>1-c'_\kappa\big|\,\tilde\Psi_p>\delta,\, Z_p>\Delta,\, \tilde\Omega_{p-1},\, \Omega'_{p-1},\, \Omega_{p,\tilde\epsilon_p}\big)\\
&\geq\mathbb{P}\big(\hat\Psi_p>1-c'_\kappa\big|\,\tilde\Omega_{p-1},\, \Omega'_{p-1},\, \Omega_{p,\tilde\epsilon_p}\big)\\
&\quad+\mathbb{P}\big(\tilde\Psi_p>\delta,\, Z_p>\Delta\big|\,\tilde\Omega_{p-1},\, \Omega'_{p-1},\, \Omega_{p,\tilde\epsilon_p}\big)-1\\
&\geq\mathbb{P}\big(\hat\Psi_p>1-c'_\kappa\big|\,\tilde\Omega_{p-1},\, \Omega'_{p-1},\, \Omega_{p,\tilde\epsilon_p}\big)+\mathbb{P}\big(\tilde\Psi_p>\delta\big|\,\tilde\Omega_{p-1},\, \Omega'_{p-1},\, \Omega_{p,\tilde\epsilon_p}\big)\\
&\quad+\mathbb{P}\big(Z_p>\Delta\big|\,\tilde\Omega_{p-1},\, \Omega'_{p-1},\, \Omega_{p,\tilde\epsilon_p}\big)-2
\end{aligned} \tag{S.23}$$

where the penultimate inequality uses Lemma S1 while the last inequality uses the fact that $\mathbb{P}(A\cap B)\geq\mathbb{P}(A)+\mathbb{P}(B)-1$ for all $A,B\in\mathcal{F}$ (Fréchet's inequality). We now find a lower bound for the each term appearing on the r.h.s. of (S.23).

To this end remark that, under C4,

$$\begin{aligned}
\tilde\Omega_{p-1}\cap\Omega'_{p-1}&=\Big\{\tilde\Omega_{p-1},\, \Omega'_{p-1},\, \hat\mu_{p-1}\big(B_{c_\star\epsilon_{p-1}}(\theta_\star)\big)\geq\frac{\zeta_4}{1+\zeta_3}\Big\}\\
\Omega'_{p-1}&=\Big\{\Omega'_{p-1},\, \mu_{p-1}\big(B_{c_\star\epsilon_{p-1}}(\theta_\star)\big)\geq\frac{\zeta_2}{1+\zeta_1}\Big\}
\end{aligned} \tag{S.24}$$

Recall that $c_*\leq k_{\kappa/2}$ and let $\tau_p=t_p-t_{p-1}$.

Then, for the first term on the r.h.s. of (S.23), for all $p \geq 1$,

$$\begin{aligned}
&\mathbb{P}\big(\hat{\Psi}_p > 1 - c'_\kappa \big| \, \tilde{\Omega}_{p-1}, \, \Omega'_{p-1}, \, \Omega_{p,\tilde{\epsilon}_p}\big) \\
&\qquad\qquad \geq \mathbb{P}\big(\hat{\Psi}_p > 1 - c'_\kappa \big| \, \tilde{\Omega}_{p-1}, \Omega'_{p-1}\big) - \mathbb{P}(\Omega^c_{p,\tilde{\epsilon}_p}) \\
&\qquad\qquad \geq 1 - \frac{v(\zeta_4/(1+\zeta_3))}{c'_\kappa} \, \tau_p^{-1/2} - \mathbb{P}(\Omega^c_{p,\tilde{\epsilon}_p})
\end{aligned} \tag{S.25}$$

with $v()$ as in the proof of Lemma S4. The first inequality uses Lemma S1, A2, C2 and C4 while the second inequality uses in addition (S.24), Lemma S2 and Markov's inequality.

Similarly, for the second probability on the r.h.s. of (S.23) we have for all $p \geq 1$

$$\begin{aligned}
&\mathbb{P}\big(\tilde{\Psi}_p > \delta \big| \, \tilde{\Omega}_{p-1}, \, \Omega'_{p-1}, \, \Omega_{p,\tilde{\epsilon}_p}\big) \\
&\qquad\qquad \geq \mathbb{P}\big(\tilde{\Psi}_p > \delta \big| \, \tilde{\Omega}_{p-1}, \, \Omega'_{p-1}\big) - \mathbb{P}(\Omega^c_{p,\tilde{\epsilon}_p}) \\
&\qquad\qquad \geq 1 - \frac{v(\zeta_2/(1+\zeta_1))}{1-\delta} \, \tau_p^{-1/2} - \mathbb{P}(\Omega^c_{p,\tilde{\epsilon}_p}).
\end{aligned} \tag{S.26}$$

To find a lower bound for the third term on the r.h.s. of (S.23) remark first that, for all $p \geq 1$

$$\begin{aligned}
\mathbb{P}\big(Z_p > \Delta, \, \tilde{\Omega}^c_{p-1} \big| \, \Omega'_{p-1}, \, \Omega_{p,\tilde{\epsilon}_p}\big) &\leq \mathbb{P}\big(Z_p > \Delta \big| \, \tilde{\Omega}^c_{p-1}, \, \Omega'_{p-1}, \, \Omega_{p,\tilde{\epsilon}_p}\big) \\
&\leq \mathbb{P}\big(Z_p > \Delta \big| \, \tilde{\Omega}^c_{p-1}, \, \Omega'_{p-1}\big) + \mathbb{P}(\Omega^c_{p,\tilde{\epsilon}_p}) \\
&\leq \mathbb{P}\big(1 - \tilde{\Psi}_p > \Delta \big| \, \tilde{\Omega}^c_{p-1}, \, \Omega'_{p-1}\big) + \mathbb{P}(\Omega^c_{p,\tilde{\epsilon}_p}) \\
&\leq \frac{v(\zeta_2/(1+\zeta_1))}{\Delta} \, \tau_p^{-1/2} + \mathbb{P}(\Omega^c_{p,\tilde{\epsilon}_p})
\end{aligned}$$

where the second inequality uses Lemma S1, the third inequality uses the fact, since $c_\star \leq \kappa/2$, we have $\tilde{\Omega}^c_{p-1} \cap \Omega'_{p-1} \subset \Omega'_{p-1} \cap \big\{B_{\kappa\epsilon_{p-1}/2}(\theta_\star) \cap B_{(1+\kappa)\epsilon_{p-1}}(\bar{\vartheta}_{t_{p-1}}) = \varnothing\big\}$ and the last inequality uses similar computations as in (S.26).

Therefore, for all $p \geq 1$,

$$\begin{aligned}
&\mathbb{P}\big(Z_p > \Delta \big| \, \tilde{\Omega}_{p-1}, \, \Omega'_{p-1}, \, \Omega_{p,\tilde{\epsilon}_p}\big) \\
&\quad \geq \mathbb{P}\big(Z_p > \Delta, \, \tilde{\Omega}_{p-1} \big| \, \Omega'_{p-1}, \, \Omega_{p,\tilde{\epsilon}_p}\big) \\
&\quad \geq \mathbb{P}\big(Z_p > \Delta \big| \, \Omega'_{p-1}, \, \Omega_{p,\tilde{\epsilon}_p}\big) - \frac{v(\zeta_2/(1+\zeta_1))}{\Delta} \, \tau_p^{-1/2} - \mathbb{P}(\Omega^c_{p,\tilde{\epsilon}_p}).
\end{aligned} \tag{S.27}$$

Using (S.23), (S.25), (S.26), (S.27) and the fact that $\lim_{p\to+\infty} \mathbb{P}(\Omega^c_{p,\tilde{\epsilon}_p}) = 0$ we conclude that for all $c_1 \in (0,1)$ there exists a $p_{c_1} \in \mathbb{N}$ (independent of $N$ and $M$) such that $b_{p,1} \geq (1 - b_p) - c_1$ for all $p \geq p_{c_1}$.

To find a lower bound for $b_{p,2}$ note that

$$\begin{aligned}
b_{p,2} &= \mathbb{P}\big(\tilde{\Psi}_p > \delta \big| \, Z_p > \Delta, \, \Omega'_{p-1}, \, \Omega_{p,\tilde{\epsilon}_p}\big) \\
&\geq \mathbb{P}\big(\tilde{\Psi}_p > \delta \big| \, \Omega'_{p-1}, \, \Omega_{p,\tilde{\epsilon}_p}\big) - \mathbb{P}\big(Z_p \leq \Delta \big| \, \Omega'_{p-1}, \, \Omega_{p,\tilde{\epsilon}_p}\big) \\
&\geq 1 - \frac{v(\zeta_2/(1+\zeta_1))}{1-\delta} \, \tau_p^{-1/2} - \mathbb{P}(\Omega^c_{p,\tilde{\epsilon}_p}) - b_p
\end{aligned}$$

where the first inequality uses Lemma S1 while the second inequality uses (**??**) and similar computations as in (S.26). Since $\lim_{p\to+\infty}\mathbb{P}(\Omega^c_{p,\tilde{\epsilon}_p})=0$, this shows that for all $c_2\in(0,1)$ there exists a $p_{c_2}\geq 1$ (independent of $N$ and $M$) such that $b_{p,2}\geq c_2-b_p$ for all $p\geq p_{c_2}$. This concludes to show (S.20).

To conclude the proof let $c\in(0,1)$ and $f:[0,1]\to(0,+\infty)$ be the mapping defined by $f(b)=b+(1-b)(c-b)^2$, $b\in[0,1]$. Notice that $f$ is continuous an strictly positive on $[0,1]$ so that $\min_{b\in[0,1]}f(b)>0$. Therefore, using (S.13) and (S.17)-(S.20) (with $c_1=1-c$ and $c_2=c$), we have for all $p\geq \underline{p}$,

$$\begin{aligned}\mathbb{P}\big(\bar{\vartheta}_{t_p}\in B_{\epsilon_p}(\theta_\star)|\,\hat{\vartheta}_{t_{p-1}}\not\in B_{\epsilon_{p-1}}(\theta_\star),\,\Omega_{p,\tilde{\epsilon}_p}\big)&\geq \underline{c}\,\gamma^{\nu}_{t_{p-1}}\epsilon^d_{p-1}\big(b_p+(1-b_p)(c-b_p)^2\big)\\&\geq \underline{c}\,\gamma^{\nu}_{t_{p-1}}\epsilon^d_{p-1}.\end{aligned}$$

Consequently, using (S.12), for all $p\geq\underline{p}$,

$$\begin{aligned}\mathbb{P}\big(\bar{\vartheta}_{t_p}\not\in B_{\epsilon_p}(\theta_\star)|\,\bar{\vartheta}_{t_{p-1}}\not\in B_{\epsilon_{p-1}}(\theta_\star)\big)&\leq 1-\underline{c}\,\gamma^{\nu}_{t_{p-1}}\epsilon^d_{p-1}\mathbb{P}(\Omega_{p,\tilde{\epsilon}_p})\\&\leq 1-\underline{c}\,\gamma^{\nu}_{t_{p-1}}\epsilon^d_{p-1}/2\end{aligned}$$

where, since $\lim_{r\to+\infty}\mathbb{P}(\Omega^c_{r-1,r})=1$, the last inequality holds for $\underline{p}$ sufficiently large. The proof is complete. □

**Theorem S1.** *Assume A1-A7, C2 and C4. Then, there exists a constant $\bar{c}\in\mathbb{R}_{>0}$ such that*

$$\sup_{p\geq 1}p^{\varrho}\sup_{(M,N)\in\mathcal{Q}_\kappa}\mathbb{P}\big(\bar{\vartheta}_{t_p}\not\in B_{\epsilon_p}(\theta_\star)\big)\leq\bar{c}$$

*with $\mathcal{Q}_\kappa$ as in Lemma S4.*

*Proof.* Let $(M,N)\in\mathcal{Q}_\kappa$ Below $\bar{c}>0$ and $\underline{p}\geq 1$ are two finite constants (independent of $N$ and $M$) whose values can change from one expression to another

For every $p\geq 1$ we define

$$b_p=\mathbb{P}(\bar{\vartheta}_{t_p}\not\in B_{\epsilon_p}(\theta_\star)),\quad x_p=\mathbb{P}(\bar{\vartheta}_{t_p}\not\in B_{\epsilon_p}(\theta_\star)|\,\bar{\vartheta}_{t_{p-1}}\not\in B_{\epsilon_{p-1}}(\theta_\star))$$

and

$$y_p=\mathbb{P}(\bar{\vartheta}_{t_p}\not\in B_{\epsilon_p}(\theta_\star)|\,\bar{\vartheta}_{t_{p-1}}\in B_{\epsilon_{p-1}}(\theta_\star)).$$

Then, with the convention that empty products equal one, we have

$$b_p=b_0\prod_{s=1}^{p}(x_s-y_s)+\sum_{s=1}^{p}y_s\prod_{j=s+1}^{p}(x_j-y_j),\quad\forall p\geq 1 \tag{S.28}$$

and in the remainder of the proof we find an upper bound for each of the two terms on the r.h.s. of (S.28).

Remark first that (with the convention that empty sums are null)

$$t_1\,\kappa^{-2(p-1)} \le t_p \le t_1\,\kappa^{-2(p-1)} + \sum_{i=0}^{p-2} \kappa^{-2i} \le \kappa^{-2(p-1)}\big(t_1 + (\kappa^{-2}-1)^{-1}\big), \quad \forall p \ge 1 \tag{S.29}$$

so that, by Lemma S4 and using the shorthand $\tau_p = t_p - t_{p-1}$,

$$y_p \le \bar{c}\,\tau_p^{-1/2} \le \bar{c}\,\kappa^p \quad \forall p \ge 1. \tag{S.30}$$

By Lemma S5, $x_p \le 1 - \bar{c}^{-1}\gamma^{\nu}_{t_{p-1}}\epsilon^d_{p-1}$ for all $p \ge \underline{p}$. Therefore, as $\lim_{p\to+\infty} y_p = 0$ by (S.30), while $\lim_{p\to+\infty}\gamma^{\nu}_{t_{p-1}}\epsilon^d_{p-1} = 0$ under C2, it follows that

$$|x_p - y_p| \le \big|1 - \bar{c}^{-1}\gamma^{\nu}_{t_{p-1}}\epsilon^d_{p-1}\big|, \quad \forall p \ge 1.$$

Under C2, and using (S.29), $\beta > 0$ and $(\gamma_t)_{t\ge 1}$ are such that $\lim_{p\to+\infty}\epsilon_p^{\beta}/\gamma^{\nu}_{t_p} = 0$, and thus

$$|x_p - y_p| \le 1 - \tilde{\epsilon}^{d+\beta}_{p-1}, \quad \forall p \ge \underline{p} \tag{S.31}$$

where $\tilde{\epsilon}_p = \big(p^{-1}\,\varrho\log(p+1)\big)^{\frac{1}{d+\beta}}$ for every $p \ge 1$. Henceforth $\underline{p}$ is taken sufficiently large so that

$$\tilde{\epsilon}_p < \min_{1\le s<p}\tilde{\epsilon}_s, \quad \forall p \ge \underline{p}. \tag{S.32}$$

Note that such a $\underline{p}$ exists since the sequence $(\tilde{\epsilon}_p)_{p\ge 1}$ is non-increasing for $p$ large enough.

Then, for all $p > \underline{p}$ and $s \in \{\underline{p}-1,\dots,p-1\}$, we have

$$\begin{aligned}\prod_{j=s+1}^{p}|x_j - y_j| \le \exp\Big(-\sum_{j=s+1}^{p}\tilde{\epsilon}^{d+\beta}_{j-1}\Big) &\le \exp\Big(-(p-s)\,\tilde{\epsilon}^{d+\beta}_p\Big)\\ &\le \exp\Big(-\Big(1-\frac{s}{p}\Big)\log(p^{\varrho})\Big)\\ &= p^{-\varrho}\exp\Big(\frac{s}{p}\log(p^{\varrho})\Big)\end{aligned}$$

where the first inequality uses (S.31) and the second inequality uses (S.32). This shows that

$$\prod_{j=s+1}^{p}|x_j - y_j| \le \bar{c}\,p^{-\varrho}\exp\Big(\frac{s}{p}\log(p^{\varrho})\Big), \quad \forall p\ge 1, \quad \forall s \in \{0,\dots,p-1\}. \tag{S.33}$$

Applying (S.33) with $s=0$ yields, for the first term appearing on the r.h.s. of (S.28),

$$\prod_{s=1}^{p}\big|x_s - y_s\big| \le \bar{c}\,p^{-\varrho}, \quad \forall p \ge 2. \tag{S.34}$$

For the second term on the r.h.s. of (S.28) we have for all $p \geq 1$ and $s \in \{0, \dots, p-1\}$, using (S.30) and (S.33),

$$y_s \prod_{j=s+1}^{p} |x_j - y_j| \leq \bar{c}\,\kappa^s p^{-\varrho} \exp\Big(\frac{s}{p}\log(p^\varrho)\Big) = \bar{c}\,p^{-\varrho} \exp\Big( - s\Big(\log(\kappa^{-1}) - \frac{\log(p^\varrho)}{p}\Big)\Big).$$

Let $\underline{p}$ be large enough so that $\log(p^\varrho)/p \leq \log(\kappa^{-1})/2$ for all $p \geq \underline{p}$. Then, for $p \geq \underline{p}$, we have

$$\sum_{s=1}^{p} y_s \prod_{j=s+1}^{p} |x_j - y_j| \leq \bar{c}\,p^{-\varrho} \sum_{s=1}^{\infty} \exp\Big( - \frac{s}{2}\log(\kappa^{-2})\Big) \leq \bar{c}\,p^{-\varrho}. \tag{S.35}$$

Combining (S.28), (S.34) and (S.35) yields the result.

□

### S1.3.2 Under Conditions C2 and C4*

**Lemma S6.** *Assume A1-A5, C2 and C4*. Then, for every $(M, N) \in \mathcal{Q}_\kappa$ there exists a constant $\bar{c} \in \mathbb{R}_{>0}$ such that*

$$\mathbb{P}\big(\bar{\vartheta}_{t_p} \notin B_{\epsilon_p}(\theta_\star) |\, \bar{\vartheta}_{t_{p-1}} \in B_{\epsilon_{p-1}}(\theta_\star)\big) \leq \bar{c}\,(t_p - t_{p-1})^{-1/2}, \quad \forall p \in \mathbb{N}.$$

*with $\mathcal{Q}_\kappa = \{(M, N) \in \mathbb{N}^2 :\ N \geq (2K_\kappa)^d\}$, with $K_\kappa$ defined in* (S.1).

*Proof.* For every $p \geq 1$ let $\mu_{t_p} = \tilde{N}^{-1} \sum_{n=1}^{\tilde{N}} \delta_{\vartheta^n_{t_{p-1}}}$ and note that, under C4*, $\mathbb{P}(\bar{\vartheta}_{t_p} = \bar{\vartheta}^{(2)}_{t_p}) = 1$ for all $p \geq 1$, with $\bar{\vartheta}^{(2)}_{t_p}$ as in Lemma S3. For every $p \geq 1$ let $n_p \in 1 : \tilde{N}$ be such that $\bar{\vartheta}^{(2)}_{t_p} = \vartheta^{n_p}_{t_{p-1}}$ and note that $\tilde{w}^{n_p}_{t_p} \geq \tilde{N}^{-1}$.

Then, for every $p \geq 1$ we have

$$\begin{aligned}
\mathbb{P}\big(\bar{\vartheta}_{t_p} \notin B_{\epsilon_p}(\theta_\star) |\, \bar{\vartheta}_{t_{p-1}} \in B_{\epsilon_{p-1}}(\theta_\star)\big) &= \mathbb{P}\big(\bar{\vartheta}^{(2)}_{t_p} \notin B_{\epsilon_p}(\theta_\star) |\, \bar{\vartheta}_{t_{p-1}} \in B_{\epsilon_{p-1}}(\theta_\star)\big) \\
&\leq \mathbb{P}\big(\Psi_{t_{p-1}:t_p}(\mu_{t_p})(B^c_{\epsilon_p}(\theta_\star)) \geq \tilde{N}^{-1} |\, \bar{\vartheta}_{t_{p-1}} \in B_{\epsilon_{p-1}}(\theta_\star)\big) \\
&\leq \tilde{N}\,\mathbb{E}\Big[\Psi_{t_{p-1}:t_p}(\mu_{t_p})(B^c_{\epsilon_p}(\theta_\star)) |\, \bar{\vartheta}_{t_{p-1}} \in B_{\epsilon_{p-1}}(\theta_\star)\Big] \\
&\leq \tilde{N} v(c)(t_p - t_{p-1})^{-1/2}
\end{aligned}$$

with $v(\cdot)$ as in the proof of Lemma S4 and where the last inequality holds under A2, C2 and C4* and for some constant $c \in \mathbb{R}_{>0}$. The proof is complete.

□

**Lemma S7.** *Assume A1-A7, C2 and C4*. Then, there exist constants $\underline{c} \in \mathbb{R}_{>0}$ and $\bar{p} \in \mathbb{N}$ such that*

$$\sup_{(N,M) \in \mathcal{Q}_\kappa} \mathbb{P}\big(\bar{\vartheta}_{t_p} \notin B_{\epsilon_p}(\theta_\star) |\, \bar{\vartheta}_{t_{p-1}} \notin B_{\epsilon_{p-1}}(\theta_\star)\big) \leq 1 - \underline{c}\,\gamma^{\nu}_{t_{p-1}} \epsilon^d_{p-1}, \quad \forall p \geq \underline{p}$$

*with $\mathcal{Q}_\kappa$ as in Lemma S4.*

*Proof.* Under C4*, $\mathbb{P}(\bar{\vartheta}_{t_p} = \bar{\vartheta}^{(2)}_{t_p}) = 1$ for all $p \geq 1$, with $\bar{\vartheta}^{(2)}_{t_p}$ as in Lemma S3. Therefore, under A1-A7, C2 and C4*, the results is a direct consequence of Lemma S3. □

**Theorem S2.** *Assume A1-A7, C2 and C4*. Then, for every* $(M, N) \in \mathcal{Q}_\kappa$ *there exists a constant* $\bar{c} \in \mathbb{R}_{>0}$ *such that*

$$\sup_{p\geq 1} p^{\varrho} \mathbb{P}\big(\bar{\vartheta}_{t_p} \not\in B_{\epsilon_p}(\theta_\star)\big) \leq \bar{c}$$

*with* $\mathcal{Q}_\kappa$ *as in Lemma S4.*

*Proof.* The proof is identical to that of Theorem S1, where Lemma S6 and S7 are used in place of Lemme S4 and S5. □

## S1.4 Preliminary results for the sequence of PPDs

### S1.4.1 Under Conditions C1 and C3

**Lemma S8.** *Assume A1-A5, C1 and C3. Then, there exists a constant* $\bar{c} \in \mathbb{R}_{>0}$ *such that, for every* $(j, p) \in \mathbb{N}^2$,

$$\sup_{(M,N)\in\mathcal{Q}_\kappa} \mathbb{P}\Big(\bar{\theta}_{t_{p+j}} \not\in B_{(\kappa^j c_j \epsilon_p)}(\theta_\star) \big| \, \hat{\theta}_{t_{p+j-1}} \in B_{(\kappa^{j-1} c_{j-1}\epsilon_p)}(\theta_\star),\ \xi_{p+j-1} = \kappa^{j-1} c_{j-1}\epsilon_p\Big)$$
$$\leq \bar{c}\Big((c_{j-1}^2\, \epsilon_p^2\, t_p)^{-1} + \kappa^j t_p^{-1/2}\Big)$$

*with* $\mathcal{Q}_\kappa$ *as in Lemma S4.*

*Proof.* Let $(M, N) \in \mathcal{Q}_\kappa$ and, for every $p \geq 1$, let $\eta_{p-1} = \frac{1}{N}\sum_{n=1}^N \delta_{\theta^n_{t_{p-1}}}$. Note that, since $N \geq (2K_\kappa)^d$, with $K_\kappa$ defined in (S.1), we have under C1

$$\mathbb{P}\Big(\hat{\theta}_{t_{p+j-1}} \in B_{(\kappa^{j-1}c_{j-1}\epsilon_p)}(\theta_\star),\ \xi_{p+j-1} = \kappa^{j-1}c_{j-1}\epsilon_p\Big)$$
$$= \mathbb{P}\Big(\hat{\theta}_{t_{p+j-1}} \in B_{(\kappa^{j-1}c_{j-1}\epsilon_p)}(\theta_\star),\ \xi_{p+j-1} = \kappa^{j-1}c_{j-1}\epsilon_r,\ \eta_{p-1}\big(B_{\kappa^{j-1}c_{j-1}\epsilon_p/K_\kappa}(\theta_\star)\big) \geq \tilde{c}K_\kappa^{-d}\Big)$$

with $\tilde{c} > 0$ as in the proof of Lemma S4.

Let $\bar{\alpha} > 0$ be as in Lemma S2, $\underline{\kappa} = \kappa\sqrt{(1 + \bar{\alpha}/2)/(1 + \bar{\alpha})}$ and note that, since $c_j \geq c_{j-1}$ for all $j \geq 1$, we have

$$\frac{(\kappa^j c_j \epsilon_p) - \underline{\kappa}(\kappa^{j-1}c_{j-1}\epsilon_p)}{\kappa^{j-1}c_{j-1}\epsilon_p} = \kappa\frac{c_j}{c_{j-1}} - \underline{\kappa} \geq \kappa - \underline{\kappa}, \quad \forall (p, j) \in \mathbb{N}^2.$$

Therefore, under the assumptions of the lemma, and using similar computations as in (S.10) and (S.11), to show the result it is enough to show that there exists a constant $\bar{c}_2 \in \mathbb{R}_{>0}$ (independent of $N$ and $M$) such that, for every $(j, p) \in \mathbb{N}^2$,

$$\mathbb{E}\Big[\Psi_{t_{p+j-1}:t_{p+j}}(\eta_{p-1})\big(B^c_{\underline{\kappa}(\kappa^{j-1}c_{j-1}\epsilon_p)}(\theta_\star)\big)\big|\eta_{p-1}\big(B_{(\kappa^{j-1}c_{j-1}\epsilon_p/K_\kappa)}(\theta_\star)\big) \geq \tilde{c}K_\kappa^{-d}\Big]$$
$$\leq \bar{c}_2\big((c_{j-1}^2\,\epsilon_r^2\,t_p)^{-1} + \kappa^j t_r^{-1/2}\big). \tag{S.36}$$

Under the assumptions of the lemma, (S.36) follows from Lemma S2 (with $\tilde{c}_j = c_j\kappa^j \in (0, 1]$ for all $j \geq 0$) and the proof is complete. □

### S1.4.2 Under Conditions C1-C4

**Lemma S9.** *Assume A1-A7 and C1-C4. Then,*

$$\sum_{p=1}^{\infty} \sup_{(M,N)\in\mathcal{Q}_\kappa} \mathbb{P}(S_p = 1) < +\infty$$

*with $\mathcal{Q}_\kappa$ as in Lemma S4 and $S_p = \mathbb{1}_{(2\epsilon_p,+\infty)}\big(\|\bar{\theta}_{t_p} - \bar{\vartheta}_{t_p}\|\big)$ for every $p \in \mathbb{N}_0$.*

*Proof.* Let $(M, N) \in \mathcal{Q}_\kappa$ and notice that, under the assumptions of the theorem, all the conditions of Theorem S1 and of Lemma S8 are verified. Below $\bar{c} \in \mathbb{R}_{>0}$ and $\underline{p} \in \mathbb{N}$ are constants (independent of $N$ and $M$) whose values can change from one expression to another,

For every $(p, j) \in \mathbb{N}_0^2$ let $\tilde{\epsilon}_{p,j} = c_j \kappa^j \epsilon_p$ and $\bar{S}_p = \inf\big\{s \geq 1 \text{ such that } S_{p+s} = 1\big\}$.

Then,

$$\begin{aligned}
\sum_{p=1}^{\infty} \sup_{(M,N)\in\mathcal{Q}_\kappa} \mathbb{P}(S_p = 1) &= \sum_{p=1}^{\infty} \sup_{(M,N)\in\mathcal{Q}_\kappa} \sum_{k=1}^{\infty} \mathbb{P}(S_p = 1,\, \bar{S}_p = k) \\
&= \sum_{p=1}^{\infty} \sup_{(M,N)\in\mathcal{Q}_\kappa} \sum_{k=1}^{\infty} \mathbb{P}(S_p = 1,\, \bar{\vartheta}_{t_{p+k}} \in B_{\epsilon_{p+k}}(\theta_\star),\, \bar{S}_p = k) \\
&+ \sum_{p=1}^{\infty} \sup_{(M,N)\in\mathcal{Q}_\kappa} \sum_{k=1}^{\infty} \mathbb{P}(S_p = 1,\, \bar{\vartheta}_{t_{p+k}} \notin B_{\epsilon_{p+k}}(\theta_\star),\, \bar{S}_p = k) \qquad \text{(S.37)} \\
&\leq \sum_{p=1}^{\infty} \sup_{(M,N)\in\mathcal{Q}_\kappa} \sum_{k=1}^{\infty} \mathbb{P}(\bar{\theta}_{t_{p+k}} \notin B_{\epsilon_{p+k}}(\theta_\star),\, S_p = 1,\, \bar{S}_p = k) \\
&+ \sum_{p=1}^{\infty} \sup_{(M,N)\in\mathcal{Q}_\kappa} \sum_{k=1}^{\infty} \mathbb{P}(\bar{\vartheta}_{t_{p+k}} \notin B_{\epsilon_{p+k}}(\theta_\star))
\end{aligned}$$

and in the remainder of the proof we show that the two double series appearing on the r.h.s. of (S.37) are finite.

By Theorem S1, $p^\varrho \sup_{(M,N)\in\mathcal{Q}_\kappa} \mathbb{P}(\bar{\vartheta}_{t_p} \notin B_{\epsilon_p}(\theta_\star)) \leq \bar{c}$ so that, for the first double series in (S.37), we have

$$\begin{aligned}
\sum_{p=1}^{\infty} \sup_{(N,M)\in\mathcal{Q}_\kappa} \sum_{k=1}^{\infty} \mathbb{P}(\bar{\vartheta}_{t_{p+k}} \notin B_{\epsilon_{p+k}}(\theta_\star)) &\leq \bar{c} \sum_{p=1}^{\infty}\sum_{k=1}^{\infty} \frac{1}{(p+k)^\varrho} \\
&\leq \bar{c} \sum_{p=1}^{\infty}\sum_{k=1}^{\infty} \frac{1}{(p^2+k^2)^{\varrho/2}} \qquad \text{(S.38)} \\
&\leq \bar{c}
\end{aligned}$$

where the last inequality holds because $\varrho > 2$ (see e.g. Borwein and Borwein, 1987, p.305).

We now study the second double series in (S.37). To this end let $\underline{p} \geq 1$ be large enough so that, for all $p \geq \underline{p}$, we have $\tilde{\epsilon}_{p,j} \leq \epsilon_{p+j}$ for all $j \geq 1$. Remark that such a $\underline{p}$ exists because $\sup_{j\geq 1} c_j \kappa^j < 1$ while $\lim_{p\to+\infty} \epsilon_p/\epsilon_{p-1} = 1$. Then, for all $p \geq \underline{p}$,

$$\begin{aligned}\sum_{k=1}^{\infty} \mathbb{P}(\bar{\theta}_{t_{p+k}} &\notin B_{\epsilon_{p+k}}(\theta_\star),\, S_p = 1,\, \bar{S}_p = k)\\ &\leq \mathbb{P}(\bar{\theta}_{t_{p+1}} \notin B_{\tilde{\epsilon}_{p,1}}(\theta_\star),\, S_p = 1,\, \bar{S}_p = 1)\\ &+ \sum_{k=2}^{\infty} \mathbb{P}(\bar{\theta}_{t_{p+k}} \notin B_{\tilde{\epsilon}_{p,k}}(\theta_\star),\, S_p = 1,\, \bar{S}_p = k).\end{aligned} \tag{S.39}$$

Below we find an upper bound for the two terms on the r.h.s. of (S.39).

For the first term we have, for all $p \geq \underline{p}$,

$$\begin{aligned}&\mathbb{P}(\bar{\theta}_{t_{p+1}} \notin B_{\tilde{\epsilon}_{p,1}}(\theta_\star),\, S_p = 1,\, \bar{S}_p = 1)\\ &\quad= \mathbb{P}(\bar{\theta}_{t_{p+1}} \notin B_{\tilde{\epsilon}_{p,1}}(\theta_\star),\, \bar{\vartheta}_{t_p} \in B_{\epsilon_p}(\theta_\star),\, \hat{\theta}_{t_p} = \bar{\vartheta}_{t_p},\, \xi_p = \epsilon_p,\, S_p = 1,\, \bar{S}_p = 1)\\ &\quad+ \mathbb{P}(\bar{\theta}_{t_{p+1}} \notin B_{\tilde{\epsilon}_{p,1}}(\theta_\star),\, \bar{\vartheta}_{t_p} \notin B_{\epsilon_p}(\theta_\star),\, S_p = 1,\, \bar{S}_p = 1)\\ &\quad\leq \mathbb{P}\big(\bar{\theta}_{t_{p+1}} \notin B_{\tilde{\epsilon}_{p,1}}(\theta_\star) \big| \,\hat{\theta}_{t_p} \in B_{\epsilon_p}(\theta_\star),\, \xi_p = \epsilon_p\big) + \mathbb{P}(\bar{\vartheta}_{t_p} \notin B_{\epsilon_p}(\theta_\star))\\ &\quad\leq \bar{c}\big(\epsilon_p^{-2} t_p^{-1} + t_p^{-1/2} + p^{-\varrho}\big)\end{aligned} \tag{S.40}$$

where the last inequality uses Theorem S1 and Lemma S8, and the fact that $\epsilon_p = \tilde{\epsilon}_{p,0}$.

We now find an upper bound for the second term on the r.h.s. of (S.39). For every $k \geq 2$ we have

$$\big\{S_p = 1,\, \bar{S}_p = k\big\} \subset \big\{\xi_{p+j} = \tilde{\epsilon}_{p,j},\, \hat{\theta}_{p+j} = \bar{\theta}_{p+j}\big\} \quad \forall j = 1, \dots, (k-1)$$

and therefore, for all $p \geq 1$ and $k \geq 2$,

$$\begin{aligned}&\mathbb{P}(\bar{\theta}_{t_{p+k}} \notin B_{\tilde{\epsilon}_{p,k}}(\theta_\star),\, S_p = 1,\, \bar{S}_p = k)\\ &= \mathbb{P}(\bar{\theta}_{t_{p+k}} \notin B_{\tilde{\epsilon}_{p,k}}(\theta_\star),\, S_p = 1,\, \bar{S}_p = k,\, \hat{\theta}_{t_{p+k-1}} \in B_{\tilde{\epsilon}_{p,k-1}}(\theta_\star),\, \xi_{p+k-1} = \tilde{\epsilon}_{p,k-1})\\ &+ \mathbb{P}(\bar{\theta}_{t_{p+k}} \notin B_{\tilde{\epsilon}_{p,k}}(\theta_\star),\, S_p = 1,\, \bar{S}_p = k,\, \hat{\theta}_{t_{p+k-1}} \notin B_{\tilde{\epsilon}_{p,k-1}}(\theta_\star),\, \hat{\theta}_{t_{p+k-1}} = \bar{\theta}_{t_{p+k-1}})\\ &\leq \mathbb{P}(\bar{S}_p = k,\, \bar{\theta}_{t_{p+k}} \notin B_{\tilde{\epsilon}_{p,k}}(\theta_\star) \big| \,\hat{\theta}_{t_{p+k-1}} \in B_{\tilde{\epsilon}_{p,k-1}}(\theta_\star),\, \xi_{p+k-1} = \tilde{\epsilon}_{p,k-1})\\ &+ \mathbb{P}(\bar{\theta}_{t_{p+k-1}} \notin B_{\tilde{\epsilon}_{p,k-1}}(\theta_\star),\, S_p = 1,\, \bar{S}_p = k).\end{aligned}$$

To proceed further we define, for every $(p, j, k) \in \mathbb{N}^3$,

$$b_{j,k,p} = \mathbb{P}\big(\bar{S}_p = k,\, \bar{\theta}_{t_{p+j}} \notin B_{\tilde{\epsilon}_{p,j}}(\theta_\star) \big| \hat{\theta}_{t_{p+j-1}} \in B_{\tilde{\epsilon}_{p,j-1}}(\theta_\star),\, \xi_{p+j-1} = \tilde{\epsilon}_{p,j-1}\big)$$

so that, for all $p \geq 1$,

$$\begin{aligned}\sum_{k=2}^{\infty} \mathbb{P}(\bar{\theta}_{t_{p+k}} &\notin B_{\tilde{\epsilon}_{p,k}}(\theta_\star),\, S_p = 1,\, \bar{S}_p = k)\\ &\leq \sum_{k=2}^{\infty}\sum_{j=2}^{k} b_{j,k,p} + \sum_{k=2}^{\infty} \mathbb{P}(\bar{\theta}_{t_{p+1}} \notin B_{\tilde{\epsilon}_{p,1}}(\theta_\star), S_p = 1,\, \bar{S}_p = k).\end{aligned} \tag{S.41}$$

For the first double series on the r.h.s. of (S.41) we have, for every $p \geq 1$ and $\bar{k} \in \mathbb{N}$,

$$\begin{aligned}
\sum_{k=2}^{\bar{k}} \sum_{j=2}^{k} b_{j,k,p} &= \sum_{j=2}^{\bar{k}} \sum_{k=j}^{\bar{k}} b_{j,k,p} \\
&\leq \sum_{j=2}^{\bar{k}} \sum_{k=1}^{\infty} b_{j,k,p} \\
&= \sum_{j=2}^{\bar{k}} \mathbb{P}\big(\bar{\theta}_{t_{p+j}} \notin B_{\tilde{\epsilon}_{p,j}}(\theta_\star) \big|\, \hat{\theta}_{t_{p+j-1}} \in B_{\tilde{\epsilon}_{p,j-1}}(\theta_\star),\, \xi_{p+j-1} = \tilde{\epsilon}_{p,j-1}\big) \\
&\leq \bar{c}\bigg( \frac{1}{\epsilon_p^2 t_p} \sum_{j=1}^{\infty} c_{j-1}^{-2} + t_p^{-\frac{1}{2}} \sum_{j=1}^{\infty} \kappa^j \bigg)
\end{aligned}$$

where the last inequality uses Lemma S8. Therefore, because $\sum_{j=1}^{\infty} c_{j-1}^{-2} < +\infty$ and $\sum_{j=1}^{\infty} \kappa^j < +\infty$, it follows that

$$\sum_{k=2}^{\infty} \sum_{j=2}^{k} b_{j,k,p} \leq \bar{c}\big(\epsilon_p^{-2} t_p^{-1} + t_p^{-\frac{1}{2}}\big). \tag{S.42}$$

To prepare bounding the second double series on the r.h.s. of (S.41) note that, for all $p \geq 1$ and $k \geq 2$, we have

$$\begin{aligned}
&\mathbb{P}(\bar{\theta}_{t_{p+1}} \notin B_{\tilde{\epsilon}_{p,1}}(\theta_\star),\, S_p = 1,\, \bar{S}_p = k) \\
&\quad = \mathbb{P}(\bar{\theta}_{t_{p+1}} \notin B_{\tilde{\epsilon}_{p,1}}(\theta_\star),\, S_p = 1,\, \bar{S}_p = k,\, \hat{\theta}_{t_p} = \bar{\vartheta}_{t_p},\, \xi_p = \epsilon_p) \\
&\quad \leq \mathbb{P}(\bar{S}_p = k,\, \bar{\theta}_{t_{p+1}} \notin B_{\tilde{\epsilon}_{p,1}}(\theta_\star) \big|\, \hat{\theta}_{t_p} \in B_{\epsilon_p}(\theta_\star),\, \xi_p = \epsilon_p) + \mathbb{P}(\bar{\vartheta}_{t_p} \notin B_{\epsilon_p}(\theta_\star),\, \bar{S}_p = k)
\end{aligned}$$

so that

$$\begin{aligned}
&\sum_{k=2}^{\infty} \mathbb{P}\big(\bar{\theta}_{t_{p+1}} \notin B_{\tilde{\epsilon}_{p,1}}(\theta_\star),\, S_p = 1,\, \bar{S}_p = k\big) \\
&\qquad \leq \mathbb{P}\big(\bar{\vartheta}_{t_p} \notin B_{\epsilon_p}(\theta_\star)\big) + \mathbb{P}\big(\bar{\theta}_{t_{p+1}} \notin B_{\tilde{\epsilon}_{p,1}}(\theta_\star) \big|\, \hat{\theta}_{t_p} \in B_{\epsilon_p}(\theta_\star),\, \zeta_p = \epsilon_p\big) \\
&\qquad \leq \bar{c}\,\big(p^{-\varrho} + \big(\epsilon_p^{-2} t_p^{-1} + t_p^{-1/2}\big)\big)
\end{aligned} \tag{S.43}$$

where the last inequality uses Theorem S1 and Lemma S8.

Therefore, by (S.39)-(S.43),

$$\sum_{k=1}^{\infty} \mathbb{P}(\bar{\theta}_{t_{p+k}} \notin B_{\epsilon_{p+k}}(\theta_\star),\, S_p = 1,\, \bar{S}_p = k) \leq \bar{c}\big(\epsilon_p^{-2}\, t_p^{-1} + t_p^{-1/2} + p^{-\varrho}\big), \quad \forall p \geq \underline{p}$$

and thus, since $\sum_{p=1}^{\infty} \epsilon_p^{-2}\, t_p^{-1} < +\infty$ and $\sum_{p=1}^{\infty} t_p^{-1/2} < +\infty$, it follows that

$$\sum_{p=1}^{\infty} \sup_{(M,N) \in \mathcal{Q}_\kappa} \sum_{k=1}^{\infty} \mathbb{P}(\bar{\theta}_{t_{p+k}} \notin B_{\epsilon_{p+k}}(\theta_\star),\, S_p = 1,\, \bar{S}_p = k) \leq \bar{c}.$$

Together with (S.37) and (S.38), this shows the result. □

### S1.4.3 Under Conditions C1-C3 and C4*

**Lemma S10.** *Assume A1-A7, C1-C3 and C4*. Then, for every* $(M, N) \in \mathcal{Q}_\kappa$

$$\sum_{p=1}^{\infty} \mathbb{P}(S_p = 1) < +\infty$$

*with* $\mathcal{Q}_\kappa$ *as in Lemma S4 and* $S_p$ *as in Lemma S9.*

*Proof.* The proof of this result is similar to that of Lemma S9, where Theorem S2 is used in placed of Theorem S1. □

## S2 Proof of Theorem 1

*Proof of Theorem 1.* Below we only prove the first part of the theorem since, to prove the second part, it suffices to replace Theorem S1 by Theorem S2 and Lemma S9 by Lemma S10 in what follows.

Let $M$ and $N$ be as in the statement of the theorem. Then, $(M, N) \in \mathcal{Q}_\kappa$, with $\mathcal{Q}_\kappa$ as in Lemma S4. Therefore, under the assumptions made in the first part of the theorem, all the conditions of Theorem S1 and of Lemma S9 are fulfilled.

Let $S_p : \Omega \to \{0, 1\}$ be as in the statement of Lemma S9 and $\Omega_1 \in \mathcal{F}$ be a set of $\mathbb{P}$-probability one such that, for all $\omega \in \Omega_1$,

$$p_\omega := \inf\big\{p \geq 1 : \ S_{p+k}(\omega) = 0, \forall k \in \mathbb{N}_0\big\} < +\infty, \quad \lim_{p\to+\infty} \hat{\theta}^\omega_{t_p} = \theta_\star. \tag{S.44}$$

Note that such a set exists by Theorem S1 and Lemma S9.

Let $\Omega_2 \in \mathcal{F}$ be a set of $\mathbb{P}$-probability one such that, for every $\omega \in \Omega_2$, we have

$$\theta^n_{t_p}(\omega) \in B_{\xi_p(\omega)}(\hat{\theta}^\omega_{t_p}), \quad \forall n \in 1:N, \quad \forall p \in \mathbb{N}. \tag{S.45}$$

Note that, because $N \geq 2^d$, such a set exists under C1.

As a first step we show that there exist constants $C \in \mathbb{R}$ and $\tilde{p} \in \mathbb{N}$ such that, for every $\omega \in \tilde{\Omega} := \Omega_1 \cap \Omega_2$, we have

$$\|\hat{\theta}^\omega_{t_p} - \theta_\star\| \leq C\, p^{\frac{1+\varepsilon}{2}} t_p^{-1/2}, \quad \forall p \geq p_\omega + \tilde{p}. \tag{S.46}$$

To show (S.46) let $\omega \in \tilde{\Omega}$. Then,

$$\|\hat{\theta}^\omega_{t_p} - \theta_\star\| \leq 2 \sum_{k=p}^{\infty} \xi_k(\omega), \quad \forall p \geq p_\omega. \tag{S.47}$$

Indeed, $\omega$ is such that, for all $p \geq p_\omega$, (S.45) holds while $\hat{\theta}^\omega_{t_p} = \bar{\theta}^\omega_{t_p}$, and thus (S.47) is necessary condition to have $\lim_{p\to+\infty} \hat{\theta}^\omega_{t_p} = \theta_\star$.

To proceed further let $\underline{k} \geq 1$ be such that $c_k = k^{(1+\varepsilon)/2}$ for all $k \geq \underline{k}$. Then, for all $p \geq p_\omega + \underline{k} + 1$, we have

$$\begin{aligned}
\sum_{k=p}^{\infty} \xi_k(\omega) &= \epsilon_{p_\omega} \sum_{k=p}^{\infty} c_{k-p_\omega} \kappa^{k-p_\omega} \\
&= \epsilon_{p_\omega} \sum_{k=p}^{\infty} (k-p_\omega)^{\frac{1+\varepsilon}{2}} \kappa^{k-p_\omega} \\
&= \epsilon_{p_\omega} \kappa^{p-p_\omega} \sum_{k=0}^{\infty} (k+p-p_\omega)^{\frac{1+\varepsilon}{2}} \kappa^{k} \\
&= \epsilon_{p_\omega} \kappa^{p-p_\omega} \sum_{k=0}^{\infty} \exp\left(\frac{(1+\varepsilon)}{2} \log(k+p-p_\omega) - k\log(\kappa^{-1})\right) \\
&\leq \epsilon_{p_\omega} (p-p_\omega)^{\frac{1+\varepsilon}{2}} \kappa^{p-p_\omega} \sum_{k=0}^{\infty} \exp\left(k\left(\frac{1+\varepsilon}{2(p-p_\omega)} - \log(\kappa^{-1})\right)\right)
\end{aligned} \tag{S.48}$$

where the last inequality uses the fact that $\log(x+y) \leq \log(y) + \frac{x}{y}$ for all $x \geq 0$ and $y > 0$.

Let $\tilde{p} = (1+\varepsilon)\log(\kappa^{-1})^{-1} + \underline{k} + 2$ so that

$$\frac{1+\varepsilon}{2(p-p_\omega)} \leq \frac{1}{2}\log(\kappa^{-1}), \quad \forall p \geq \tilde{p}_\omega + \tilde{p}.$$

Note also that, using (S.29),

$$\kappa^{p-p_\omega} \leq t_p^{-1/2}\big((\kappa^{-2}-1)^{-1} + t_{p_\omega}\big)^{1/2}, \quad \forall p \geq \tilde{p}_\omega + \tilde{p}.$$

Therefore, using (S.48), we have

$$2\sum_{k=p}^{\infty} \xi_k(\omega) \leq p^{\frac{1+\varepsilon}{2}} t_p^{-1/2} C_1, \quad \forall p \geq \tilde{p}_\omega + \tilde{p} \tag{S.49}$$

with

$$C_1 = \sup_{p\geq 1} 2\big((\kappa^{-2}-1)^{-1} + t_p\big)^{\frac{1}{2}} \epsilon_p \kappa^{-p} \sum_{k=0}^{\infty} \exp\Big(-\frac{k}{2}\log(\kappa^{-1})\Big) < +\infty. \tag{S.50}$$

Note that $C_1$ is indeed finite since, by (S.48), $t_p = \mathcal{O}(\kappa^{-2p})$. Together with (S.47), (S.49) shows (S.46).

To proceed further remark that, by (S.45) and (S.46), for for every $\omega \in \tilde{\Omega}$ we have

$$\max_{n\in 1:N} \|\theta_{t_p}^{n,\omega} - \theta_\star\| \leq 3C_1\, p^{\frac{1+\varepsilon}{2}} t_p^{-1/2}, \quad \forall p \geq p_\omega + \tilde{p} \tag{S.51}$$

implying that, for every $\omega \in \tilde{\Omega}$,

$$\tilde{\pi}_t^{N,\omega}\Big(\big\{\theta \in \Theta : \|\theta - \theta_\star\| \geq 4C_1\, p^{\frac{1+\varepsilon}{2}} t_p^{-1/2}\big\}\Big) = 0,\ \forall t \in (t_p+1) : t_{p+1},\ \forall p \geq p_\omega + \tilde{p}. \tag{S.52}$$

To conclude the proof note that, for every $p \geq 2$,

$$\begin{aligned} p^{\frac{1+\varepsilon}{2}} t_p^{-1/2} &= \log(t)^{\frac{1+\varepsilon}{2}} t^{-1/2}\, \frac{p^{\frac{1+\varepsilon}{2}} t_p^{-1/2}}{\log(t)^{\frac{1+\varepsilon}{2}} t^{-1/2}} \\ &\leq \log(t)^{\frac{1+\varepsilon}{2}} t^{-1/2} \left(\frac{p}{\frac{1}{2}\log(t_1) + (p-2)\log(\kappa^{-1})}\right)^{\frac{1+\varepsilon}{2}} (t_p^{-1}\, t_{p+1})^{1/2} \\ &\leq C_2\, \log(t)^{\frac{1+\varepsilon}{2}} t^{-1/2} \end{aligned} \tag{S.53}$$

where the penultimate inequality uses (S.29) and where

$$C_2 = \sup_{p>2} \left(\frac{p}{\frac{1}{2}\log(t_1) + (p-2)\log(\kappa^{-1})}\right)^{\frac{1+\varepsilon}{2}} (t_p^{-1} t_{p+1})^{1/2} < +\infty. \tag{S.54}$$

Together with (S.52), (S.53) shows that for every $\omega \in \tilde{\Omega}$

$$\tilde{\pi}_t^{N,\omega}\Big(\big\{\theta \in \Theta : \|\theta - \theta_\star\| \geq 4C_1\, C_2\, \log(t)^{\frac{1+\varepsilon}{2}} t^{-1/2}\big\}\Big) = 0, \quad \forall t \geq t_{p_\omega + \tilde{p}}. \tag{S.55}$$

The proof is complete upon noting that $\mathbb{P}(\tilde{\Omega}) = \mathbb{P}(\Omega_1 \cap \Omega_2) = 1$ as $\mathbb{P}(\Omega_1) = \mathbb{P}(\Omega_2) = 1$. □

## S3 Proof of Theorem 2

*Proof of Theorem 2.* By assumption $N^{-1}\sum_{n=1}^N \theta_0^n \neq \theta_\star$ and $\tilde{N}^{-1}\sum_{n=1}^{\tilde{N}} \vartheta_0^n \neq \theta_\star$ and thus

$$\mathbb{P}\big(\forall p \geq 1, \hat{\theta}_{t_p}^N \neq \theta_\star,\ \bar{\vartheta}_{t_p} \neq \theta_\star\big) = 1.$$

Consequently, under C1* (resp. C2*), for any $p \geq 1$, $\epsilon > 0$ and $N \geq 2^d$, with probability one the set $\theta_{t_p}^{1:N}$ (resp. $\vartheta_{t_p}^{1:\tilde{N}}$) contains at least one point in $B_{\epsilon/K_\kappa}(\theta_\star)$ whenever $\hat{\theta}_{t_p} \in B_\epsilon(\theta_\star)$ (resp. $\bar{\vartheta}_{t_p} \in B_\epsilon(\theta_\star)$), with $K_\kappa$ as in Lemma S2. This simple observation readily shows that Theorems S1- S2 and Lemmas S9-S10 hold when, instead of being as defined in Lemma S4, the set $\mathcal{Q}_\kappa$ is defined by $\mathcal{Q}_\kappa = \{(M,N) \in \mathbb{N}^2 :\ N \geq K_\kappa^d\}$. The result then follows from the computations made in the proof of Theorem 1. □

## S4 Proof of Corollary 1

*Proof of Corollary 1.* Below we only prove the result under C1-C4. To prove the result under C1-C3 and C4* it suffices to replace Theorem S1 by Theorem S2 and Lemma S9 by Lemma S10 in what follows. The result under the additional conditions C1* and C2* follows from a similar argument as the one used in the proof of Theorem 2.

Let $(M,N)\in\mathcal{Q}_\kappa$, with $\mathcal{Q}_\kappa$ as in Lemma S4, and $\tilde\Omega\in\mathcal{F}$ with $\mathbb{P}(\tilde\Omega)=1$ be as in the proof of Theorem 1.

Then, by (S.51), for all $\omega\in\tilde\Omega$ we have

$$\|\hat\theta^{N,\omega}_{t_p}-\theta_\star\|\leq 3C_1\,p^{\frac{1+\varepsilon}{2}}t_p^{-1/2},\quad \forall p\geq p_\omega+\tilde p$$

with $(p_\omega,\tilde p)\in\mathbb{N}$ and $C_1\in\mathbb{R}$ as in the proof of Theorem 1.

Consequently, using the fact that (S.45) and (S.49) hold for every $\omega\in\tilde\Omega$, it follows that for every $\omega\in\tilde\Omega$, $p\geq p_\omega+\tilde p$ and $t\in\{t_p+1,\dots,t_{p+1}-1\}$ we have

$$\|\hat\theta^{N,\omega}_{t}-\theta_\star\|\leq \|\hat\theta^{N,\omega}_{t_p}-\theta_\star\|+\xi_p(\omega)\leq 3C_1\,p^{\frac{1+\varepsilon}{2}}t_p^{-1/2}+\xi_p(\omega)\leq 4C_1\,p^{\frac{1+\varepsilon}{2}}t_p^{-1/2}.$$

Together with (S.53), this shows that for every $\omega\in\tilde\Omega$

$$\|\hat\theta^{N,\omega}_{t}-\theta_\star\|\leq 4C_1\,C_2\,,\log(t)^{\frac{1+\varepsilon}{2}}t^{-1/2},\quad \forall t\geq t_{p_\omega+\tilde p}\tag{S.56}$$

and the proof is complete □

# S5 Proof of Theorem 3

*Proof of Theorem 3.* Below we only prove the result under C1-C4, the result under the additional conditions C1* and C2* then follows from a similar argument as the one used in the proof of Theorem 2.

Let $\Omega_1\in\mathcal{F}$ with $\mathbb{P}(\Omega_1)=1$ be such that, for all $\omega\in\Omega_1$,

$$\lim_{p\to+\infty}\hat\theta^{\omega}_{t_p}=\theta_\star,\quad \forall (M,N)\in\mathcal{Q}_\kappa.$$

Note that such a set exists by Theorem S1 and Lemma S9. Let $\Omega_2\in\mathcal{F}$ be such that $\mathbb{P}(\Omega_2)=1$ and such that (S.45) holds for all $\omega\in\Omega_2$ and all $(M,N)\in\mathcal{Q}_\kappa$.

Let $(M,N)\in\mathcal{Q}_\kappa$ and, for every $p\geq 1$ let $S_p$ be as in the statement of Lemma S9 and $\Omega_p^{(N,M)}=\{S_{p'}=0,\,\forall p'\geq p\}$. For $\omega\in\Omega$ let

$$p_\omega^{(N,M)}:=\inf\big\{p\geq 1:\ S_{p+k}(\omega)=0,\,\forall k\in\mathbb{N}_0\big\}$$

and remark that $\Omega_p^{(N,M)}=\{p_\omega^{(N,M)}\leq p\}$.

Let $\Omega'\in\mathcal{F}$ be such that $\mathbb{P}(\Omega')=1$ and such that (S.55) holds for every $(M,N)\in\mathcal{Q}_\kappa$. Then, the computations in the proof of Theorem 1 shows that

$$\tilde\Omega_p^{(N,M)}:=\Omega_1\cap\Omega_2\cap\Omega_p^{(N,M)}\subset\Omega'$$

and thus, by (S.55) and (S.56), for every $\omega\in\tilde\Omega_p^{(N,M)}$ we have

$$\tilde\pi_t^{N,\omega}\Big(\big\{\theta\in\Theta:\ \|\theta-\theta_\star\|\geq 4C_1\,C_2\,\log(t)^{\frac{1+\varepsilon}{2}}t^{-1/2}\big\}\Big)=0,\quad \forall t\geq t_{p+\tilde p}\geq t_{p_\omega^{(N,M)}+\tilde p}$$

and

$$\|\hat\theta^{N,\omega}_{t}-\theta_\star\|\leq 4C_1\,C_2\,\log(t)^{\frac{1+\varepsilon}{2}}t^{-1/2}\quad \forall t\geq t_{p+\tilde p}\geq t_{p_\omega^{(N,M)}+\tilde p}$$

where $\tilde{p} \in \mathbb{N}$ is as in (S.55) while $C_1$ and $C_2$ are defined in (S.50) and (S.54), respectively.

Since $\mathbb{P}(\tilde{\Omega}_p^{(N,M)}) = \mathbb{P}(\Omega_p^{(N,M)})$, this shows that

$$\mathbb{P}\Big(\sup_{t\geq t_p} \tilde{\pi}_t^N\big(\{\theta \in \Theta:\ \|\theta-\theta_\star\| \geq 4C_1\, C_2\, \log(t)^{\frac{1+\varepsilon}{2}} t^{-1/2}\}\big)=0\Big) = \mathbb{P}(\Omega_{p-\tilde{p}}^{(N,M)}), \quad \forall p > \tilde{p}$$

and

$$\mathbb{P}\Big(\sup_{t\geq t_p} \log(t)^{-\frac{1+\varepsilon}{2}} t^{1/2} \|\hat{\theta}_t^N - \theta_\star\| \leq 4C_1C_2\Big) = \mathbb{P}(\Omega_{p-\tilde{p}}^{(N,M)}), \quad \forall p > \tilde{p}$$

where, for every $(M,N) \in \mathcal{Q}_\kappa$ and $p \geq 1$,

$$\begin{aligned}\mathbb{P}\big(\Omega_p^{(N,M)}\big) = 1 - \mathbb{P}\big(\exists p' \geq p,\, S_{p'} = 1\big) &\geq 1 - \sum_{p'=p}^{\infty} \mathbb{P}(S_{p'} = 1)\\ &\geq 1 - \sum_{p'=p}^{\infty} \sup_{(M,N)\in\mathcal{Q}_\kappa} \mathbb{P}(S_{p'} = 1).\end{aligned}$$

By Lemma S9, $\lim_{p\to+\infty} \sum_{p'=p}^{\infty} \sup_{(M,N)\in\mathcal{Q}_\kappa} \mathbb{P}(S_{p'} = 1) = 0$ and thus

$$\lim_{p\to+\infty} \inf_{(M,N)\in\mathcal{Q}_\kappa} \mathbb{P}\Big(\sup_{t\geq t_p} \tilde{\pi}_t^N\big(\{\theta \in \Theta:\ \|\theta-\theta_\star\| \geq 4C_1\, C_2\, \log(t)^{\frac{1+\varepsilon}{2}} t^{-1/2}\}\big)=0\Big) = 1$$

$$\lim_{p\to+\infty} \inf_{(M,N)\in\mathcal{Q}_\kappa} \mathbb{P}\Big(\sup_{t\geq t_p} \log(t)^{-\frac{1+\varepsilon}{2}} t^{1/2} \|\hat{\theta}_t^\omega - \theta_\star\| \leq 4C_1C_2\Big) = 1.$$

The proof is complete.

□

# S6 Proof of Lemme S2 and S3

## S6.1 Two direct implications of Assumptions A1, A2 and A5

**Lemma S11.** *Assume A1 and A5. Then,*

$$-\mathbb{E}\Big[\log \frac{f_\theta}{f_{\theta_\star}}(Y_1)\Big] = \frac{1}{2}(\theta-\theta_\star)^T V_{\theta_\star}(\theta-\theta_\star) + o(\|\theta-\theta_\star\|^2), \quad (\theta \to \theta_\star)$$

*with* $V_{\theta_\star} = -\frac{\partial^2}{\partial\theta\partial\theta^T}\mathbb{E}[\log f_{\theta_\star}(Y_1)]$*. Moreover, the equality* $V_{\theta_\star} = -\mathbb{E}[\ddot{l}_{\theta_\star}(Y_1)]$*, with* $\ddot{l}_{\theta_\star}$ *as in A5, holds and* $V_{\theta_\star}$ *is a* $d\times d$ *positive-definite matrix.*

*Proof.* The result is a direct consequence of A1 and A5, and the proof is omitted to save space. □

For a $d \times d$ matrix $A$ let $A_{i,j}$ be its entry $(i,j)$. We then have the following result.

**Lemma S12.** *Assume A1, A2 and A5 and let* $V_{\theta_\star}$ *be as in Lemma S11. Then, for every* $\epsilon > 0$ *there exists a constant* $v_\epsilon \in \mathbb{R}_{>0}$ *such that*

$$\lim_{t\to+\infty} \mathbb{P}\Big(\max_{(i,j)\in\{1,\dots,d\}^2} \sup_{\theta\in B_{v_\epsilon}(\theta_\star)} \Big|\frac{1}{t}\sum_{s=1}^{t} \ddot{l}_\theta(Y_s)_{ij} - (-V_{\theta_\star})_{ij}\Big| \geq \epsilon\Big) = 0.$$

*Proof.* Let $\dddot{m}_{\theta_\star}$ be as in A5 and $v_\epsilon \in \mathbb{R}_{>0}$ be such that we have both $B_{v_\epsilon}(\theta_\star) \subset U$ and $v_\epsilon \leq \epsilon(4\mathbb{E}[\dddot{m}_{\theta_\star}(Y_1)])^{-1}$, with $U$ as in A5. Notice that such a $v_\epsilon$ exists since, under A5, we have $\mathbb{E}[\dddot{m}_{\theta_\star}(Y_1)] < +\infty$. Note also that

$$\begin{aligned}
&\mathbb{P}\Big(\max_{(i,j)\in\{1,\dots,d\}^2}\sup_{\theta\in B_{v_\epsilon}(\theta_\star)}\Big|\frac{1}{t}\sum_{s=1}^t \ddot{l}_\theta(Y_s)_{ij} - (-V_{\theta_\star})_{ij}\Big| \geq \epsilon\Big)\\
&\qquad\qquad \leq \mathbb{P}\Big(\max_{(i,j)\in\{1,\dots,d\}^2}\sup_{\theta\in B_{v_\epsilon}(\theta_\star)}\Big|\frac{1}{t}\sum_{s=1}^t \ddot{l}_\theta(Y_s)_{ij} - \frac{1}{t}\sum_{s=1}^t \ddot{l}_{\theta_\star}(Y_s)_{ij}\Big| \geq \epsilon/2\Big)\\
&\qquad\qquad + \sum_{(i,j)\in\{1,\dots,d\}^2}\mathbb{P}\Big(\Big|\frac{1}{t}\sum_{s=1}^t \ddot{l}_{\theta_\star}(Y_s)_{ij} - \mathbb{E}[\ddot{l}_{\theta_\star}(Y_1)]_{ij}\Big| \geq \epsilon/2\Big)
\end{aligned}$$

where, under A2 and A5, and by the law of large numbers, the last term converges to zero as $t \to +\infty$. To show that the first term also converges to 0 as $t \to +\infty$ note that, under A5 and using the mean value theorem,

$$\max_{(i,j)\in\{1,\dots,d\}^2}\sup_{\theta\in B_{v_\epsilon}(\theta_\star)}\Big|\frac{1}{t}\sum_{s=1}^t \ddot{l}_\theta(Y_s)_{ij} - \frac{1}{t}\sum_{s=1}^t \ddot{l}_{\theta_\star}(Y_s)_{ij}\Big| \leq v_\epsilon \frac{1}{t}\sum_{s=1}^t \dddot{m}_{\theta_\star}(Y_s), \quad \mathbb{P}-a.s.$$

Thus,

$$\begin{aligned}
&\mathbb{P}\Big(\max_{(i,j)\in\{1,\dots,d\}^2}\sup_{\theta\in B_{v_\epsilon}(\theta_\star)}\Big|\frac{1}{t}\sum_{s=1}^t \ddot{l}_\theta(Y_s)_{ij} - \frac{1}{t}\sum_{s=1}^t \ddot{l}_{\theta_\star}(Y_s)_{ij}\Big| \geq \frac{\epsilon}{2}\Big)\\
&\qquad\qquad \leq \mathbb{P}\Big(v_\epsilon \frac{1}{t}\sum_{s=1}^t \dddot{m}_{\theta_\star}(Y_s) \geq \frac{\epsilon}{2}\Big)\\
&\qquad\qquad \leq \mathbb{P}\Big(v_\epsilon\Big|\frac{1}{t}\sum_{s=1}^t \dddot{m}_{\theta_\star}(Y_s) - \mathbb{E}[\dddot{m}_{\theta_\star}(Y_1)]\Big| \geq \frac{\epsilon}{2} - v_\epsilon\mathbb{E}[\dddot{m}_{\theta_\star}(Y_1)]\Big)\\
&\qquad\qquad \leq \mathbb{P}\Big(\Big|\frac{1}{t}\sum_{s=1}^t \dddot{m}_{\theta_\star}(Y_s) - \mathbb{E}[\dddot{m}_{\theta_\star}(Y_1)]\Big| \geq \frac{\epsilon}{4}\Big)
\end{aligned}$$

where the penultimate inequality uses the fact that $v_\epsilon \leq \epsilon(4\mathbb{E}[\dddot{m}_{\theta_\star}(Y_1)])^{-1}$. Under A2 and A5, and by the law of large numbers, the last probability converges to zero as $t \to +\infty$. The proof is complete. □

## S6.2 Proof of Lemma S2

We first proof the following lemma which is a direct consequence of Kleijn and van der Vaart (2012, Theorem 3.3).

**Lemma S13.** *Assume A1-A5. Then, there exist constants* $(\epsilon_\star, \delta_\star, D, \tilde{D}) \in \mathbb{R}^4_{>0}$ *such that, for all sequence* $(M_t)_{t\geq 1}$ *in* $\mathbb{R}_{>0}$ *verifying* $\lim_{t\to+\infty} M_t = +\infty$ *and* $\lim_{t\to+\infty} M_t t^{-1/2} = 0$,

*there exists a sequence of tests $(\psi_t)_{t\geq 1}$ such that*

$$\mathbb{E}\big[\psi_t(Y_{1:t})\big] \leq \tilde{D}^{-1}\Big(t^{-1/2} + \frac{e^{-\tilde{D}M_t}}{\sqrt{M_t}}\Big), \quad \forall t \geq 1$$

*while, for every $t \geq 1$ such that $M_t^{-1} \leq \delta_*$ and $\theta \in \Theta$ such that $\|\theta - \theta_\star\| \geq M_t t^{-1/2}$, we have*

$$\mu_\theta^t\big(1 - \psi_t(Y_{1:t})\big) \leq e^{-t\,D(\|\theta-\theta_\star\|^2 \wedge \epsilon_\star^2)}$$

*with the measure $\mu_\theta^t$ defined in A4.*

*Proof.* This result is a direct consequence of Kleijn and van der Vaart (2012, Theorem 3.3).

To show the result we need to explicit the sequence $(\psi_t)_{t\geq 1}$ used in the proof of Kleijn and van der Vaart (2012, Theorem 3.3), noticing that under A1-A5 and by Lemma S11, all the assumptions of this latter are verified.

To this end, for $L > 0$ let $\dot{l}_{\theta_\star}^L : \mathcal{Y} \to \mathbb{R}^d$ be such that, for all $y \in \mathcal{Y}$ and $i \in 1:d$, $\big(\dot{l}_{\theta_\star}^L(y)\big)_i = L$ if $\big|\big(\dot{l}_{\theta_\star}^L(y)\big)_i\big| \geq L$ and $\big(\dot{l}_{\theta_\star}^L(y)\big)_i = \big(\dot{l}_{\theta_\star}(y)\big)_i$ otherwise.

For every $t \geq 1$ let $\psi_{1,t}^L : \mathcal{Y}^t \to \{0, 1\}$ be defined by

$$\psi_{1,t}^L(y) = \mathbb{1}\Big(\Big\|\frac{1}{t}\sum_{s=1}^t \dot{l}_{\theta_\star}^L(y_s) - \mathbb{E}[\dot{l}_{\theta_\star}^L(Y_1)]\Big\| > \sqrt{M_t/t}\Big), \quad y \in \mathcal{Y}^t.$$

Then, (see the proof of Kleijn and van der Vaart, 2012, Theorem 3.3), for small enough finite constants $c_1 > 0$, $\delta_* > 0$ and $\epsilon_* > 0$ and large enough finite constant $L_* > 0$, we have

$$\mu_\theta^t\big((1 - \psi_{1,t}^{L_*}(Y_{1:t}))\big) \leq e^{-c_1 t\|\theta-\theta_\star\|}, \quad \forall \theta \in \big\{\theta' \in \Theta :\, M_t/\sqrt{t} \leq \|\theta' - \theta_\star\| \leq \epsilon_*\big\}$$

for all $t$ such that $M_t^{-1} \leq \delta_*$. We note from the computations in the proof of Kleijn and van der Vaart (2012, Theorem 3.3) that the constants $c_1$, $\delta_*$, $\epsilon_*$ and $L_*$ can be made independent of the sequence $(M_t)_{t\geq 1}$.

Next, by Kleijn and van der Vaart (2012, Lemma 3.3), there exists a sequence of tests $(\psi_{2,t})_{t\geq 1}$ and constants $(c_2, c_3) \in \mathbb{R}_{>0}^2$ such that

$$\mathbb{E}\big[\psi_{2,t}(Y_{1:t})\big] \leq e^{-tc_2}, \qquad \sup_{\{\theta:\, \|\theta-\theta_\star\|>\epsilon_*\}} \mu_\theta^t\big((1 - \psi_{2,t}(Y_{1:t})\big) \leq e^{-tc_3}, \quad \forall t \geq 1.$$

Notice that $c_2$ and $c_3$ do not depend on $(M_t)_{t\geq 1}$.

Let t $D = c_1 \wedge c_3$ and, for every $t \geq 1$, let $\psi_t = \psi_{1,t}^{L_*} \vee \psi_{2,t}$ so that the sequence $(\psi_t)_{t\geq 1}$ verifies the second part of the lemma.

To show that this sequence also verifies the first part of the lemma we define, for $i = 1, \ldots, d$,

$$X_{t,i} = \sqrt{t}\frac{\frac{1}{t}\sum_{s=1}^t \big(\dot{l}_{\theta_\star}^{L_*}(Y_s)\big)_i - \mathbb{E}\big[\big(\dot{l}_{\theta_\star}^{L_*}(Y_1)\big)_i\big]}{\sigma_i}, \quad \sigma_i = \sqrt{\mathbb{E}\big[\big(\dot{l}_{\theta_\star}^{L_*}(Y_1)\big)_i^2\big] - \mathbb{E}\big[\big(\dot{l}_{\theta_\star}^{L_*}(Y_1)\big)_i\big]^2}.$$

Then, as $\sup_{y\in\mathcal{Y}}\|\dot{l}_{\theta_\star}^{L_*}(y)\|\leq L_*<+\infty$, we have by the Berry-Esseen theorem [**reference?**]

$$\max_{i\in\{1,\dots,d\}}\sup_{x\in\mathbb{R}}\Big|\mathbb{P}\big(X_{t,i}\leq x\big)-\Phi(x)\Big|\leq c_4\,t^{-1/2},\quad \forall t\geq 1$$

for some constant $c_4\in\mathbb{R}$ and where $\Phi:\mathbb{R}\to(0,1)$ denotes the c.d.f. of the $\mathcal{N}_1(0,1)$ distribution. Let $\bar{\sigma}=\min_{i\in 1:d}\sigma_i$. Then,

$$\begin{aligned}
\mathbb{E}[\psi_{1,t}^{L_*}(Y_{1:t})]&=\mathbb{P}\Big(\sqrt{t}\,\Big\|\frac{1}{t}\sum_{s=1}^{t}\dot{l}_{\theta_\star}^{L_*}(Y_s)-\mathbb{E}[\dot{l}_{\theta_\star}^{L_*}(Y_1)]\Big\|>\sqrt{M_t}\Big)\\
&\leq\sum_{i=1}^{d}\mathbb{P}\big(|X_{t,i}|>\sqrt{M_t}\sigma_i^{-1}\big)\\
&=\sum_{i=1}^{d}\mathbb{P}\big(X_{t,i}>\sqrt{M_t}\sigma_i^{-1}\big)+\sum_{i=1}^{d}\mathbb{P}\big(X_{t,i}<-\sqrt{M_t}\sigma_i^{-1}\big)\\
&\leq 2\,\frac{d\,c_4}{t^{1/2}}+2\Phi\big(-\sqrt{M_t}/\bar{\sigma}\big)\\
&\leq 2\,\frac{d\,c_4}{t^{1/2}}+2\frac{\bar{\sigma}\,e^{-\frac{M_t}{2\bar{\sigma}^2}}}{\sqrt{M_t 2\pi}}
\end{aligned}$$

where the last inequality uses the fact that

$$\Phi(-x)=1-\Phi(x)\leq\frac{e^{-x^2/2}}{x\sqrt{2\pi}},\quad\forall x\in\mathbb{R}_{>0}.$$

Therefore,

$$\mathbb{E}[\psi_t(Y_{1:t})]\leq\mathbb{E}[\psi_{1,t}^{L_*}(Y_{1:t})]+\mathbb{E}[\psi_{2,t}(Y_{1:t})]\leq 2\,\frac{d\,c_4}{t^{1/2}}+2\frac{\bar{\sigma}\,e^{-\frac{M_t}{2\bar{\sigma}^2}}}{\sqrt{M_t 2\pi}}+e^{-tc_2},\quad\forall t\geq 1$$

and the result follows by taking $\tilde{D}\in(0,(2\bar{\sigma}^2)^{-1}]$ sufficiently small. □

*Proof of Lemma S2.* The proof is based on the proof of Kleijn and van der Vaart (2012, Theorem 3.1).

Under A2 the observations $(Y_t)_{t\geq 1}$ are i.i.d. and thus, $\mathbb{P}$-almost surely,

$$\mathbb{E}\big[\Psi_{t_{p+j-1}:t_{p+j}}(\eta)\big(B^c_{\kappa_\alpha\tilde{\epsilon}_{p,j-1}}(\theta_\star)\big)\,|\,\sigma\big(Y_{1:(t_{p+j-1})}\big)\big]=\mathbb{E}\big[\Psi_{t_{p+j-1}:t_{p+j}}(\eta)\big(B^c_{\kappa_\alpha\tilde{\epsilon}_{p,j-1}}(\theta_\star)\big)\big].$$

Below we find an upper bound for the second expectation.

First, notice that under A1-A5 the assumptions of Kleijn and van der Vaart (2012, Lemma 3.1 and Lemma 3.2) are verified. These two results play a key role in what follows.

For every $(p,j)\in\mathbb{N}^2$ let $M_{p,j}=\kappa_\alpha\tau_{p,j}^{1/2}\tilde{\epsilon}_{p,j-1}$ and $\epsilon'_{p,j}=\kappa_\alpha\tilde{\epsilon}_{p,j-1}$. Then, using the fact that $\tilde{c}_j\in(0,1]$ for all $j\geq 1$ and the definition of $(t_p,\epsilon_p)_{p\geq 1}$ given in Algorithm 1, it is easily checked that

$$\lim_{p\to+\infty}M_{p,j}=+\infty,\quad\lim_{p\to+\infty}M_{p,j}\tau_{p,j}^{-1/2}=0,\quad\forall j\in\mathbb{N}\tag{S.57}$$

Thus, for every $j \in \mathbb{N}$, there exists a sequence $(M'_{t,j})_{t\geq 1}$ in $\mathbb{R}_{>0}$ such that $M'_{\tau_{p,j},j} = M_{p,j}$ for all $p \in \mathbb{N}$ and such that $\lim_{t\to+\infty} M'_{t,j} = +\infty$ and $\lim_{t\to+\infty} M'_{t,j} t^{-1/2} = 0$.

For every $j \in \mathbb{N}$ let $(\psi_t^{(j)})_{t\geq 1}$ be a sequence of tests such that the result of Lemma S13 holds for the sequence $(M'_{t,j})_{t\geq 1}$ and $W_{p,j} = \psi^{(j)}_{\tau_{p,j}}(Y_{(t_p+j-1)} : t_{p+j})$, for every $p \in \mathbb{N}$.

Let $(\delta_*, \epsilon_\star) \in \mathbb{R}^2_{>0}$ be as in Lemma S13 and $p^{(1)} \in \mathbb{N}$ be such that

$$\epsilon'_{p,j} < \epsilon_\star, \quad M^{-1}_{p,j} \leq \delta_\star, \quad \forall p \geq p^{(1)}, \quad \forall j \in \mathbb{N}.$$

Note that such a $p^{(1)}$ exists since $(\tilde{c}_j)_{j\geq 1}$ and $(t_p, \epsilon_p)_{p\geq 1}$ are such that

$$\lim_{p\to+\infty} \sup_{j\geq 1} M^{-1}_{p,j} = 0, \quad \lim_{p\to+\infty} \sup_{j\geq 1} \tilde{\epsilon}_{p,j} = 0.$$

We also define for every $\delta > 0$

$$B(\delta) = \Big\{\theta \in \Theta : -\mathbb{E}\Big[\log \frac{f_\theta}{f_{\theta_\star}}(Y_1)\Big] \leq \delta^2, \, \mathbb{E}\Big[\Big(\log \frac{f_\theta}{f_{\theta_\star}}(Y_1)\Big)^2\Big] \leq \delta^2\Big\}$$

and, for every $(p, j) \in \mathbb{N}^2$,

$$\Xi_{p,j} = \Big\{\int_\Theta \prod_{s=t_{p+j-1}+1}^{t_{p+j}} \frac{f_\theta}{f_{\theta_\star}}(Y_s)\eta(\mathrm{d}\theta) \leq \eta\big(B(a_{p,j})\big)e^{-\tau_{p,j} a^2_{p,j}(1+\lambda)}\Big\} \tag{S.58}$$

where $a_{p,j} = M\epsilon'_{p,j}$ for all $(p, j) \in \mathbb{N}^2$, $M = \sqrt{D/((1 + \alpha)(1 + \lambda))}$.

Then, for all $p \geq p^{(1)}$ and $j \geq 1$,

$$\begin{aligned}
&\mathbb{E}[\Psi_{t_{p+j-1}:t_{p+j}}(\eta)(B^c_{\epsilon'_{p,j}}(\theta_\star))] \\
&\quad = \mathbb{E}[W_{p,j}\Psi_{t_{p+j-1}:t_{p+j}}(\eta)(B^c_{\epsilon'_{p,j}}(\theta_\star))] + \mathbb{E}\big[(1 - W_{p,j})\Psi_{t_{p+j-1}:t_{p+j}}(\eta)(B^c_{\epsilon'_{p,j}}(\theta_\star))\big] \\
&\quad \leq \mathbb{E}[W_{p,j}] + \mathbb{E}\big[(1 - W_{p,j})\mathbb{1}_{\Xi^c_{p,j}}\Psi_{t_{p+j-1}:t_{p+j}}(\eta)\big(B^c_{\epsilon_\star}(\theta_\star)\big)\big] \\
&\quad + \mathbb{E}\big[(1 - W_{p,j})\mathbb{1}_{\Xi^c_{p,j}}\Psi_{t_{p+j-1}:t_{p+j}}(\eta)\big(B_{\epsilon_\star}(\theta_\star) \setminus B_{\epsilon'_{p,j}}(\theta_\star)\big)\big] + 2\mathbb{P}(\Xi_{p,j})
\end{aligned} \tag{S.59}$$

and in the remainder of this proof we find upper bounds for each term on the r.h.s. of (S.59).

Let $p^{(2)} \in \mathbb{N}$ be such

$$a^2_{p,j}(1 + \lambda) - D\epsilon^2_\star \leq -a^2_{p,j}(1 + \lambda), \quad \forall p \geq p^{(2)}, \quad \forall j \in \mathbb{N}.$$

Note that such an $p^{(2)}$ exists since, for every $(p, j) \in \mathbb{N}^2$, $\tau^{-1/2}_{p,j} M_{p,j} \leq \kappa\tilde{\epsilon}_{p,j-1} \leq \kappa\epsilon_p$ where, by assumption, $\lim_{p\to\infty} \tilde{\epsilon}_p = 0$.

Then, by (S.58) and Lemma S13, for every $p \geq p^{(1)} \vee p^{(2)}$ and $j \geq 1$, we have, under A2,

$$\begin{aligned}
\mathbb{E}\big[(1-W_{p,j})\mathbb{1}_{\Xi^c_{p,j}}\Psi_{t_{p+j-1}:t_{p+j}}(\eta)\big(B^c_{\epsilon_\star}(\theta_\star)\big)\big]
&\leq \frac{e^{\tau_{p,j}a^2_{p,j}(1+\lambda)}}{\eta\big(B(a_{p,j})\big)}\int_{B^c_{\epsilon_\star}(\theta_\star)} \mu_\theta^{\tau_{p,j}}\big(1-\psi^{(j)}_{\tau_{p,j}}(Y_{(t_{p+j-1}+1):t_{p+j}})\big)\eta(\mathrm{d}\theta)\\
&\leq \frac{e^{\tau_{p,j}(a^2_{p,j}(1+\lambda)-D\epsilon^2_\star)}}{\eta\big(B(a_{p,j})\big)}\\
&\leq \frac{e^{-\tau_{p,j}a^2_{p,j}(1+\lambda)}}{\eta\big(B(a_{\tau_{p,j}})\big)}
\end{aligned}$$

where, for any $t \geq 1$, $\mu^t_\theta$ is as in A4.

Next we find a lower bound for $\eta\big(B(a_{p,j})\big)$ by following Kleijn and van der Vaart (2012, Lemma 3.2). Under A3 and A5, and for $\|\theta-\theta_\star\|$ small enough, we have

$$-\mathbb{E}\Big[\log\frac{f_\theta}{f_{\theta_\star}}(Y_1)\Big] \leq d\|V_{\theta_\star}\|\|\theta-\theta_\star\|^2$$

and

$$\mathbb{E}\Big[\Big(\log\frac{f_\theta}{f_{\theta_\star}}(Y_1)\Big)^2\Big] \leq \mathbb{E}[m^2_{\theta_\star}(Y_1)]\|\theta-\theta_\star\|^2.$$

Then, for $\bar{\delta}>0$ small enough, $\{\theta : \|\theta-\theta_\star\| < C_\star\,\delta\} \subset B(\delta)$ for all $\delta\in(0,\bar{\delta})$ and with $C_\star = \big(\mathbb{E}[m^2_{\theta_\star}]\vee d\|V_{\theta_\star}\|\big)^{-1/2}$.

Let $p^{(3)}\in\mathbb{N}$ be such that $M\,\kappa\epsilon_{p-1} < \bar{\delta}$ for all $p \geq p^{(3)}$ and note that, as $\bar{\alpha}>0$ and $\lambda>0$ are such that

$$K_\kappa \geq \kappa^{-1}L_\star\sqrt{(1+\bar{\alpha})(1+\lambda)} = \frac{\sqrt{(1+\bar{\alpha})(1+\lambda)}}{\kappa\,C_\star\,D^{1/2}}$$

we have $M^{-1}C_\star^{-1}\,K_\kappa^{-1} \leq \sqrt{(1+\alpha)/(1+\bar{\alpha})}\kappa$. Therefore, for all $p \geq p^{(3)}$,

$$M^{-1}\bar{\delta} > \kappa\,\tilde{\epsilon}_{p,j-1} > \kappa_\alpha\tilde{\epsilon}_{p,j-1} = \sqrt{\frac{1+\alpha}{1+\bar{\alpha}}}\,\kappa\,\tilde{\epsilon}_{p,j-1} \geq M^{-1}\,C_\star^{-1}\,k_\kappa^{-1}\,\tilde{\epsilon}_{p,j-1}, \quad \forall j\in\mathbb{N}$$

and thus $a_{p,j} = M\,\kappa_\alpha\tilde{\epsilon}_{p,j-1} \in [C_\star^{-1}\,K_\kappa^{-1}\,\tilde{\epsilon}_{p,j-1},\bar{\delta})$ for all $p \geq p^{(3)}$ and $j \geq 1$. Consequently, for every $p \geq p^{(3)}$ and $j \geq 1$

$$\eta\big(B(a_{p,j})\big) \geq \eta\big(B_{C_\star a_{p,j}}(\theta_\star)\big) \geq \eta\big(B_{\tilde{\epsilon}_{p,j-1}/K_\kappa}(\theta_\star)\big)$$

and thus, for all $p \geq p^{(1)}\vee p^{(2)}\vee p^{(3)}$,

$$\mathbb{E}\big[(1-W_{p,j})\mathbb{1}_{\Xi^c_{p,j}}\Psi_{t_{p+j-1}:t_{p+j}}(\eta)\big(B^c_{\epsilon_\star}(\theta_\star)\big)\big] \leq \frac{e^{-M^2M^2_{p,j}(1+\lambda)}}{\eta\big(B_{\tilde{\epsilon}_{p,j-1}/K_\kappa}(\theta_\star)\big)}, \quad \forall j\in\mathbb{N}. \qquad \text{(S.60)}$$

Next we consider the third term on the r.h.s. of (S.59). Let $j \geq 1$ and $I_{p,j}$ be the smallest integer such that $(I_{p,j}+1)\epsilon'_{p,j} > \epsilon_\star$. Then, following the computations in Kleijn and van der Vaart (2012, Theorem 3.1) and using similar computations as per above we have, for every $p \geq p^{(1)} \vee p^{(3)}$,

$$\begin{aligned}
\mathbb{E}\Big[(1-W_{p,j})\mathbb{1}_{\Xi^c_{p,j}}\Psi_{t_{p+j-1}:t_{p+j}}(\eta)\big(B_{\epsilon_\star}(\theta_\star)\setminus B_{\epsilon'_{p,j}}(\theta_\star)\big)\Big]&\\
&\leq \sum_{i=1}^{I_{p,j}} e^{\tau_{p,j}a^2_{p,j}(1+\lambda)-\tau_{p,j}Di^2(\epsilon'_{p,j})^2}\frac{\eta\big(\{\theta:\, i\epsilon'_{p,j}\leq\|\theta-\theta_\star\|\leq(i+1)\epsilon'_{p,j}\}\big)}{\eta\big(B(a_{p,j})\big)}\\
&\leq \frac{\sum_{i=1}^{I_{p,j}} e^{\tau_{p,j}a^2_{p,j}(1+\lambda)-\tau_{p,j}Di^2(\epsilon'_{p,j})^2}}{\eta\big(B(a_{p,j}\big)}\\
&\leq \frac{\bar{c}_1\, e^{\tau_{p,j}a^2_{p,j}(1+\lambda)-\tau_{p,j}D(\epsilon'_{p,j})^2}}{\eta\big(B_{\tilde{\epsilon}_{p,j-1}/K_\kappa}(\theta_\star)\big)}
\end{aligned}$$

where $\bar{c}_1=\sum_{i=1}^\infty e^{-D(i^2-1)}<+\infty$. Then, using the definition of $M$, this shows that for every $p\geq p^{(1)}\vee p^{(2)}$,

$$\begin{aligned}
\mathbb{E}\big[(1-W_{p,j})\mathbb{1}_{\Xi^c_{p,j}}\Psi_{t_{p+j-1}:t_{p+j}}(\eta)\big(B_{\epsilon_\star}(\theta_\star)\setminus B_{\epsilon_{p,j}}(\theta_\star)\big)\big]&\\
&\leq \frac{\bar{c}_1\, e^{-\frac{D\,\alpha}{1+\alpha}M^2_{p,j}}}{\eta\big(B_{\tilde{\epsilon}_{p,j-1}/K_\kappa}(\theta_\star)\big)},\quad \forall j\in\mathbb{N}.
\end{aligned}\tag{S.61}$$

For the last term on the r.h.s. of (S.59) we have by using Kleijn and van der Vaart (2012, Lemma 3.1),

$$\mathbb{P}(\Xi_{p,j})\leq\frac{(1+\alpha)(1+\lambda)}{D\,\lambda^2M^2_{p,j}},\quad\forall(p,j)\in\mathbb{N}^2\tag{S.62}$$

and finally, by Lemma S13, for the first term on the r.h.s. of (S.59)

$$\mathbb{E}[W_{p,j}]\leq\tilde{D}^{-1}\Bigg(\tau_{p,j}^{-1/2}+\frac{e^{-\tilde{D}M_{p,j}}}{\sqrt{M_{p,j}}}\Bigg),\quad\forall(p,j)\in\mathbb{N}^2.\tag{S.63}$$

By combining (S.59)-(S.63), we have for every $p\geq p^{(1)}\vee p^{(2)}\vee p^{(3)}$ and $j\in\mathbb{N}$,

$$\begin{aligned}
&\mathbb{E}\big[\Psi_{t_{p+j-1}:t_{p+j}}(\eta)\big(B^c_{\epsilon'_{p,j}}(\theta_\star)\big)\big]\\
&\leq\tilde{D}^{-1}\tau_{p,j}^{-1/2}+\tilde{D}^{-1}\frac{e^{-\tilde{D}M_{p,j}}}{\sqrt{M_{p,j}}}+\frac{2(1+\alpha)(1+\lambda)}{D\,\lambda^2M^2_{p,j}}+\frac{e^{-\frac{D}{1+\alpha}M^2_{p,j}}+\bar{c}_1\,e^{-\frac{D\,\alpha}{1+\alpha}M^2_{p,j}}}{\eta\big(B_{\tilde{\epsilon}_{p,j-1}/K_\kappa}(\theta_\star)\big)}.
\end{aligned}\tag{S.64}$$

To conclude the proof, remark that $\lim_{p\to+\infty}\inf_{j\geq1}M^{-1}_{p,j}=+\infty$ so that there exists a $p^{(4)}\in\mathbb{N}$ such that, for all $p\geq p^{(4)}$,

$$\frac{e^{-\tilde{D}M_{p,j}}}{\sqrt{M_{p,j}}}\leq M^{-2}_{p,j},\quad\forall j\in\mathbb{N}.$$

Together with (S.64), and using the fact that $e^{-x} \le x^{-1}$ for all $x > 0$, this shows that, for every $p \ge p^{(1)} \vee p^{(2)} \vee p^{(3)} \vee p^{(4)}$,

$$\begin{aligned}
&\mathbb{E}\big[\Psi_{t_{p+j-1}:t_{p+j}}(\eta)\big(B^c_{\epsilon'_{p,j}}(\theta_\star)\big)\big]\\
&\le \tilde{D}^{-1}\tau_{p,j}^{-1/2} + M_{p,j}^{-2}\left(\tilde{D}^{-1} + \frac{2(1+\alpha)(1+\lambda)}{D\,\lambda^2} + \frac{\frac{1+\alpha}{D} + \bar{c}_1\,\frac{1+\alpha}{D\,\alpha}}{\eta\big(B_{\tilde{\epsilon}_{p,j-1}/K_\kappa}(\theta_\star)\big)}\right), \quad \forall j \ge 1
\end{aligned}$$

and the result follows. □

## S6.3 Proof of Lemma S3

We start with some additional notation that will be used in the proof of Lemma S3.

### S6.3.1 Additional notation

Let $U \subset \Theta$ be as in A5 and, for every $p \in \mathbb{N}$, let $\tau_p = t_p - t_{p-1}$, $L_p : \Theta \times \mathcal{Y}^{\tau_p} \to \mathbb{R}$, and $H_p : \times\mathcal{Y}^{\tau_p} \to \mathbb{R}^{d\times d}$ be respectively defined by

$$L_p(\theta, y) = \frac{1}{\tau_p}\sum_{s=1}^{\tau_p} \log f_\theta(y_s), \quad (\theta, y) \in \Theta \times \mathcal{Y}^{\tau_p}, \tag{S.65}$$

and

$$H_p(\theta, y) = -\frac{1}{\tau_p}\sum_{s=1}^{\tau_p} \ddot{l}_\theta(y_s), \quad (\theta, y) \in U \times \mathcal{Y}^{\tau_p}. \tag{S.66}$$

For every $(p, \omega) \in \mathbb{N} \times \Omega$, let

$$Y^{\omega,p} = \big(Y_s(\omega),\, s \in \{t_{p-1}+1, \dots, t_p\}\big), \quad Y^p = \big(Y_s,\, s \in \{t_{p-1}+1, \dots, t_p\}\big),$$

and, for every $\epsilon > 0$ and $\delta > 0$, and with $\tilde{U}$ as in A7, let

$$U_{p,\epsilon}(y) = \Big\{\theta \in B_\epsilon(\theta_\star) : L_p(\theta, y) \ge K_{p,\epsilon}(y)\Big\}, \quad K_{p,\epsilon}(y) = \sup_{\theta \in \tilde{U}\setminus B_\epsilon(\theta_\star)} L_p(\theta, y), \tag{S.67}$$

and

$$\Omega_{p,\epsilon,\delta} = \Omega' \cap \Omega^{(1)}_{p,\epsilon} \cap \Omega^{(2)}_{p} \cap \Omega^{(3)}_{p,\delta} \cap \Omega^{(4)}_{p,\delta} \cap \Omega^{(5)}_{p,\delta} \tag{S.68}$$

where $\Omega' \in \mathcal{F}$ is such that $\mathbb{P}(\Omega') = 1$ and such that (14) in A5 holds for all $\omega \in \Omega'$,

$$
\begin{aligned}
\Omega^{(1)}_{p,\epsilon} &= \Big\{\omega \in \Omega : \hat{\theta}_{\tau_p,\mathrm{mle}}(Y^{\omega,p}) \in B_\epsilon(\theta_\star)\Big\},\\
\Omega^{(2)}_{p} &= \Big\{\omega \in \Omega : \max_{(i,j)\in\{1,\dots,d\}^2} \Big|\frac{1}{\tau_p}\sum_{s=t_{p-1}+1}^{t_p} \ddot{l}_{\theta_\star}(Y^{\omega,p}_s)_{ij} - \mathbb{E}[\ddot{l}_{\theta_\star}(Y_1)]_{ij}\Big| \leq \delta_p\Big\}\\
\Omega^{(3)}_{p,\delta} &= \Big\{\omega \in \Omega : \max_{(i,j)\in\{1,\dots,d\}^2} \sup_{\theta\in B_{v_\delta}(\theta_\star)} \Big|\frac{1}{\tau_p}\sum_{s=\tau_{p-1}}^{t_p} \ddot{l}_{\theta}(Y^{\omega,p}_s)_{ij} - (V_{\theta_\star})_{ij}\Big| \leq \delta\Big\}, \qquad \text{(S.69)}\\
\Omega^{(4)}_{p,\delta} &= \Big\{\omega \in \Omega : \sup_{\theta\in\Theta}\big|L_p(\theta, Y^{\omega,p}) - \mathbb{E}[\log f_\theta(Y_1)]\big| \leq \delta\Big\},\\
\Omega^{(5)}_{p,\delta} &= \Big\{\omega \in \Omega : \frac{1}{\tau_p}\sum_{s=t_{p-1}+1}^{t_p} \dddot{m}_{\theta_\star}(Y^{\omega,r}_s) \leq \mathbb{E}[\dddot{m}_{\theta_\star}(Y_1)] + \delta\Big\}.
\end{aligned}
$$

In (S.69), $\ddot{l}_{\theta_\star}$ and $\dddot{m}_{\theta_\star}$ are as in A5, $V_{\theta_\star}$ is as in Lemma S11 and, for every $t \in \mathbb{N}$ and $y \in \mathcal{Y}^t$, $\hat{\theta}_{t,\mathrm{mle}}(y)$, is as in A7. In the definition of $\Omega^{(3)}_{p,\delta}$, $v_\delta$ is as in the statement Lemma S12 (for $\epsilon = \delta$) while, in the definition of $\Omega^{(2)}_p$, $(\delta_p)_{p\geq 1}$ is a sequence in $\mathbb{R}_{>0}$ such that $\lim_{p\to+\infty} \delta_p = 0$ and

$$
\lim_{p\to+\infty} \mathbb{P}\bigg(\Big\{\omega \in \Omega : \max_{(i,j)\in\{1,\dots,d\}^2} \Big|\frac{1}{\tau_p}\sum_{s=t_{p-1}+1}^{t_p} \ddot{l}_{\theta_\star}(Y^{\omega,p}_s)_{ij} - \mathbb{E}[\ddot{l}_{\theta_\star}(Y_1)]_{ij}\Big| \leq \delta_r\Big\}\bigg) = 1.
$$

Note that such as sequence $(\delta_p)_{p\geq 1}$ exists under A2 and A6 since $(t_p)_{p\geq 0}$ is such that $\lim_{p\to+\infty}(t_p - t_{p-1}) = +\infty$.

The following lemma is a direct consequence of Assumptions A1-A7 and of Lemma S12.

**Lemma S14.** *Assume A2-A7, let $\delta > 0$ and $(\tilde{\epsilon}_p)_{p\geq 0}$ be a sequence in $\mathbb{R}_{>0}$ such that $\lim_{p\to+\infty}(t_p - t_{p-1})^{1/2}\tilde{\epsilon}_p = +\infty$. Then, $\lim_{p\to+\infty} \mathbb{P}(\Omega_{p,\tilde{\epsilon}_p,\delta}) = 1$.*

### S6.3.2 Proof of the lemma

*Proof of the Lemma S3.* Let $\delta > 0$ be sufficiently small so that, for every $p \geq 1$ and $\omega \in \Omega^{(3)}_{p,\delta}$, the mapping $\theta \mapsto L_p(\theta, Y^{\omega,p})$ is strictly concave on $B_{v_\delta}(\theta_\star)$. Note that such a $\delta > 0$ exists because $-V_{\theta_\star}$ is negative definite by Lemma S11. Without loss of generality we assume below that $\tilde{U} \subset B_{v_\delta}(\theta_\star)$.

Let $(\epsilon'_p)_{p\geq 1}$ be a sequence in $\mathbb{R}_{>0}$ such that $\lim_{p\to+\infty}(t_p - t_{p-1})^{1/2}\epsilon'_p = +\infty$ and $\lim_{p\to+\infty} \epsilon'_p/\tilde{\epsilon}_p = 0$, and let $\Omega_p = \Omega_{p,\epsilon'_p,\delta}$. We assume henceforth that $p$ is such that $\epsilon'_p < \tilde{\epsilon}_p/2$.

We start by first showing that

$$
\bigcup_{n=1}^{M} \big\{\omega \in \Omega_p : \vartheta^{N+n}_{t_p-1}(\omega) \in U_{p,\tilde{\epsilon}_p}(Y^{\omega,p})\big\} \subset \big\{\omega \in \Omega_p : \bar{\vartheta}^{(2)}_{t_p}(\omega) \in B_{\tilde{\epsilon}_p}(\theta_\star)\big\} \qquad \text{(S.70)}
$$

so that, $\mathbb{P}$-almost surely,

$$\begin{aligned}&\mathbb{P}\big(\bar{\vartheta}^{(2)}_{t_p}\in B_{\tilde{\epsilon}_p}(\theta_\star)\,|\,\Omega_p,\,\sigma\big(Y_{1:t_p},\vartheta^{1:\tilde{N}}_{t_0:t_{p-2}},\,\theta^{1:N}_{t_0:t_{p-1}}\big)\big)\\&\geq\mathbb{P}\Big(\exists n\in 1:M\text{ s.t. }\vartheta^{N+n}_{t_{p-1}}\in U_{p,\tilde{\epsilon}_p}(Y^p)\,|\,\Omega_p,\,\sigma\big(Y_{1:t_p},\vartheta^{1:\tilde{N}}_{t_0:t_{p-2}},\,\theta^{1:N}_{t_0:t_{p-1}}\big)\Big).\end{aligned}\tag{S.71}$$

In the remainder of the proof we show (S.70) and study probability appearing in the r.h.s. of (S.71).

For (S.70) to hold, it suffices by the definition of $\bar{\vartheta}^{(2)}_{t_p}$ to show that

$$L_p(\theta,Y^{\omega,p})\geq L_p(\theta',Y^{\omega,p}),\tag{S.72}$$

for all $(\theta,\theta')\in U_{p,\tilde{\epsilon}_p}(Y^{\omega,p})\times\Theta\setminus B_{\tilde{\epsilon}_p}(\theta_\star)$, but by the definitions of $K_{p,\tilde{\epsilon}_p}$ and $U_{p,\tilde{\epsilon}_p}$, we only need show (S.72) for $(\theta,\theta')\in U_{p,\tilde{\epsilon}_p}(Y^{\omega,p})\times\Theta\setminus\tilde{U}$.

For a sufficiently small $\delta>0$ there exists an open neighbourhood $U_\delta\subset\tilde{U}$ of $\theta_\star$ such that

$$\inf_{\theta\in U_\delta}\mathbb{E}[\log f_\theta(Y_1)]\geq 3\delta+\sup_{\theta\in\Theta\setminus\tilde{U}}\mathbb{E}[\log f_\theta(Y_1)],$$

because, under A5, the mapping $\theta\mapsto\mathbb{E}[\log f_\theta(Y_s)]$ is continuous on $\tilde{U}$ and, under A1, $\mathbb{E}[\log f_{\theta_\star}(Y_1)]>\mathbb{E}[\log f_\theta(Y_1)]$ for all $\theta\in\Theta\setminus\{\theta_\star\}$. Consequently, for every $\omega\in\Omega_p\subset\Omega^{(4)}_{p,\delta}$,

$$\begin{aligned}\inf_{\theta\in U_\delta}L_p(\theta,Y^{\omega,p})\geq\inf_{\theta\in U_\delta}\mathbb{E}[\log f_\theta(Y_1)]-\delta&\geq 2\delta+\sup_{\theta\in\Theta\setminus\tilde{U}}\mathbb{E}[\log f_\theta(Y_1)]\\&\geq\delta+\sup_{\theta\in\Theta\setminus\tilde{U}}L_r(\theta,Y^{\omega,p}),\end{aligned}$$

and because $U_{p,\tilde{\epsilon}_p}(Y^{\omega,p})\subset U_\delta$, we conclude that (S.72) holds for $(\theta,\theta')\in U_{p,\tilde{\epsilon}_p}(Y^{\omega,p})\times\Theta\setminus\tilde{U}$, whenever $p$ is sufficiently large so that $B_{\tilde{\epsilon}_p}(\theta_\star)\subset U_\delta$. Hence we also have (S.70) and (S.71).

Next we show there exists $c_\star\in\mathbb{R}_{>0}$ such that, that for sufficiently large $p$,

$$\Big\{\omega\in\Omega:\,B_{c_\star\tilde{\epsilon}_p}(\theta_\star)\subset U_{p,\tilde{\epsilon}_p}(Y^{\omega,p})\Big\}\cap\Omega_p=\Omega_p.\tag{S.73}$$

To simplify the notation in what follows let $\hat{\theta}^\omega_{p,\text{mle}}=\hat{\theta}_{\tau_p,\text{mle}}(Y^{\omega,p})$ and $H^\omega_p=H_p(\hat{\theta}^\omega_{p,\text{mle}},Y^{\omega,p})$. As preliminary computations to establish (S.73) we first show that there exists a sequence $(v_p)_{p\geq1}$ in $\mathbb{R}_{>0}$ such that $\lim_{p\to+\infty}v_p/\tilde{\epsilon}_p^2=0$ and such that, for $p$ large enough,

$$\left|L_p(\theta,Y^{\omega,p})-L_p(\hat{\theta}^\omega_{p,\text{mle}},Y^{\omega,p})+\frac{(\theta-\hat{\theta}_{p,\text{mle}})^TV_{\theta_\star}(\theta-\hat{\theta}^\omega_{p,\text{mle}})}{2}\right|\leq v_p\tag{S.74}$$

for all $(\omega,\theta)\in\Omega_p\times\overline{B_{\tilde{\epsilon}_p}(\theta_\star)}$, with $\overline{B_{\tilde{\epsilon}_p}(\theta_\star)}$ the closure of $B_{\tilde{\epsilon}_p}(\theta_\star)$.

Let $\theta\in\overline{B_{\tilde{\epsilon}_p}(\theta_\star)}$ and let us consider, for $\omega\in\Omega_p$, a second order Taylor expansion of $L_p(\theta,Y^{\omega,p})$ at $\hat{\theta}^\omega_{p,\text{mle}}$. We assume henceforth that $p$ is such that $B_{\epsilon'_p}(\theta_\star)\cap\tilde{U}=B_{\epsilon'_p}(\theta_\star)$.

Then, for $\omega \in \Omega_p \subset \Omega^{(1)}_{p,\epsilon'_p} \cap \Omega^{(3)}_{p,\delta}$, $\hat\theta^\omega_{p,\mathrm{mle}}$ is an interior extremal point of a concave function so that the first order term must be zero. Therefore, for every $\omega \in \Omega_p$,

$$L_p(\theta, Y^{\omega,p}) = L_p(\hat\theta^\omega_{p,\mathrm{mle}}, Y^{\omega,p}) - \frac{1}{2}(\theta - \hat\theta^\omega_{p,\mathrm{mle}})^T H^\omega_p(\hat\theta^\omega_p - \hat\theta^\omega_{p,\mathrm{mle}}) + R^{\omega,p}_1(\theta) \tag{S.75}$$

where, for some constant $\bar c < +\infty$ and because $\Omega_p \subset \Omega^{(1)}_{p,\tilde\epsilon_p/2} \cap \Omega^{(5)}_{p,\delta}$ (recall that $p$ is such that $\epsilon'_p < \tilde\epsilon_p/2$) the remainder $R^{\omega,p}_1(\theta)$ is such that

$$\left|R^{\omega,p}_1(\theta)\right| \le \bar c \,\|\theta - \hat\theta^\omega_{p,\mathrm{mle}}\|^3 \le \bar c\,(3\tilde\epsilon_p/2)^3. \tag{S.76}$$

Moreover, for every $(i,j) \in \{1,\dots,d\}^2$ and $\omega \in \Omega_p$, the mean value theorem yields

$$\frac{1}{t_p - t_{p-1}} \sum_{s=t_{p-1}+1}^{t_p} \ddot l_{\hat\theta^\omega_{p,\mathrm{mle}}}(Y^{\omega,p}_s)_{ij} = \frac{1}{t_p - t_{p-1}} \sum_{s=t_{p-1}+1}^{t_p} \ddot l_{\theta_\star}(Y^{\omega,p}_s)_{ij} + \tilde R^{\omega,p}_{i,j} \tag{S.77}$$

where, as $\Omega_p \subset \Omega^{(1)}_{p,\tilde\epsilon_p/2} \cap \Omega^{(5)}_{p,\delta}$ and by assuming $\bar c$ sufficiently large,

$$\left|\tilde R^{\omega,p}_{i,j}\right| \le \bar c \|\hat\theta^\omega_{p,\mathrm{mle}} - \theta_\star\| \le \bar c\,\tilde\epsilon_p. \tag{S.78}$$

Let $\tilde R^{\omega,p} = (\tilde R^{\omega,p}_{i,j})^d_{i,j=1}$. Then, by (S.66) and (S.77)

$$H^\omega_p = -\mathbb{E}[\ddot l_{\theta_\star}(Y_1)] - \tilde R^{\omega,p} - \frac{1}{t_p - t_{p-1}} \sum_{s=t_{p-1}+1}^{t_p} \ddot l_{\theta_\star}(Y^{\omega,p}_s) + \mathbb{E}[\ddot l_{\theta_\star}(Y_1)].$$

Hence by (S.78) and the fact that $\Omega_p \subset \Omega^{(2)}_p$, we have for every $\omega \in \Omega_p$,

$$\begin{aligned}
&(\theta - \hat\theta^\omega_{p,\mathrm{mle}})^T(-\mathbb{E}[\ddot l_{\theta_\star}(Y_1)])(\theta - \hat\theta^\omega_{p,\mathrm{mle}}) - d^2\bar c\,\tilde\epsilon_p^3 - d^2\tilde\epsilon_p^2\delta_p\\
&\quad\le (\theta - \hat\theta^\omega_{p,\mathrm{mle}})^T H^\omega_p(\theta - \hat\theta^\omega_{p,\mathrm{mle}})\\
&\quad\le (\theta - \hat\theta^\omega_{p,\mathrm{mle}})^T(-\mathbb{E}[\ddot l_{\theta_\star}(Y_1)])(\theta - \hat\theta^\omega_{p,\mathrm{mle}}) + d^2\bar c\,\tilde\epsilon_p^3 + d^2\tilde\epsilon_p^2\delta_p.
\end{aligned} \tag{S.79}$$

By Lemma S11, $\mathbb{E}[\ddot l_{\theta_\star}(Y_1)] = -V_{\theta_\star}$ and therefore, letting $v_p = \bar c\,(3\tilde\epsilon_p/2)^3 + \frac{1}{2}\big(d^2\bar c\,\tilde\epsilon_p^3 + d^2\tilde\epsilon_p^2\delta_p\big)$ and noting that $\lim_{pr\to+\infty} v_p/\tilde\epsilon_r^2 = 0$, (S.75), (S.76) and (S.79) show (S.74).

Next, for every $\omega \in \Omega_p$ let $\theta^{p,\omega} \in \{\theta \in \Theta : \|\theta - \theta_\star\| = \tilde\epsilon_p\}$ be such that $L_p(\theta^{p,\omega}, Y^{\omega,p}) = K_{p,\tilde\epsilon_p}(Y^{\omega,p})$. Note that such a $\theta^{p,\omega}$ exists since the set $\tilde U \setminus B_{\tilde\epsilon_p}(\theta_\star)$ is compact and, under A5 and for every $\omega \in \Omega_p \subset \Omega^{(1)}_{p,\epsilon'_p} \cap \Omega^{(3)}_{p,\delta}$, the mapping $\theta \mapsto L_p(\theta, Y^{\omega,p})$ is strictly concave on $\tilde U$ and attains its maximum on $B_{\epsilon'_p}(\theta_\star) \subset B_{\tilde\epsilon_p/2}(\theta_\star)$.

Then, by (S.74) and using the fact that, by Lemma S11, $V_{\theta_\star}$ is positive definite, for $p$ large enough and every $\omega \in \Omega_p$, we have

$$\begin{aligned}
K_{p,\tilde\epsilon_p}(Y^{\omega,p}) &\le L_p(\hat\theta^\omega_{p,\mathrm{mle}}, Y^{\omega,p}) - \frac{(\theta^{p,\omega} - \hat\theta_{p,\mathrm{mle}})^T V_{\theta_\star}(\theta^{p,\omega} - \hat\theta^\omega_{p,\mathrm{mle}})}{2} + v_p\\
&\le L_p(\hat\theta^\omega_p, Y^{\omega,p}) - \frac{\sigma_{\min}(V_{\theta_\star})}{8}\tilde\epsilon_p^2 + v_p
\end{aligned} \tag{S.80}$$

where $\sigma^2_{\min}(V_{\theta_\star}) > 0$ is the smallest eigenvalue of $V_{\theta_\star}$.

To proceed further let $c \in (0,1)$ and $\tilde\theta \in B_{c\tilde\epsilon_p}(\theta_\star)$. Then, by (S.74), for $p$ large enough and every $\omega \in \Omega_p$,

$$\begin{aligned} L_p(\tilde\theta, Y^{\omega,p}) &\geq L_p(\hat\theta^\omega_{p,\text{mle}}, Y^{\omega,p}) - \frac{(\tilde\theta - \hat\theta_{p,\text{mle}})^T V_{\theta_\star}(\tilde\theta - \hat\theta^\omega_{p,\text{mle}})}{2} - v_p \\ &\geq L_p(\hat\theta^\omega_{p,\text{mle}}, Y^{\omega,p}) - \frac{1}{2}\|\tilde\theta - \hat\theta^\omega_{p,\text{mle}}\|^2 \, \|V_{\theta_\star}\| - v_p \\ &\geq L_p(\hat\theta^\omega_{p,\text{mle}}, Y^{\omega,p}) - \frac{1}{2}\|\tilde\theta - \theta_\star\|^2 \, \|V_{\theta_\star}\| - \frac{1}{2}(\epsilon'_p)^2 - v_r \\ &\geq L_p(\hat\theta^\omega_{p,\text{mle}}, Y^{\omega,p}) - \frac{1}{2}(c\,\tilde\epsilon_p^2)\|V_{\theta_\star}\| - v'_p \end{aligned} \tag{S.81}$$

with $v'_p = \frac{1}{2}\|V_{\theta_\star}\|(\epsilon'_p)^2 + v_p$. Note that $\lim_{p\to+\infty} v'_p/\tilde\epsilon_p^2 = 0$.

Therefore, by (S.80) and (S.81), for $p$ large enough and all $\omega \in \Omega_p$, a sufficient condition to have $L_p(\tilde\theta, Y^{\omega,p}) > K_{p,\tilde\epsilon_p}(Y^{\omega,p})$ for every $\tilde\theta \in B_{c\tilde\epsilon_p}(\theta_\star)$ is that

$$c^2 < \frac{\sigma_{\min}(V_{\theta_\star})}{4\|V_{\theta_\star}\|} - \frac{2}{\|V_{\theta_\star}\|}\,\frac{v_p + v'_p}{\tilde\epsilon_p^2}.$$

Therefore, since $\lim_{p\to+\infty}(v_p+v'_p)/\tilde\epsilon_p^2 = 0$, this shows (S.73) for $c_\star = \sqrt{\sigma_{\min}(V_{\theta_\star})/(8\|V_{\theta_\star}\|)}$.

To complete the proof let $\Omega'_p = \big\{\omega \in \Omega : \, B_{c_\star\tilde\epsilon_p}(\theta_\star) \subset U_{p,\tilde\epsilon_p}(Y^{\omega,p})\big\}$ so that, by (S.71) and (S.73), for $p$ large enough and $\mathbb{P}$-almost surely,

$$\begin{aligned} &\mathbb{P}\big(\bar\vartheta^{(2)}_{t_p} \in B_{\tilde\epsilon_p}(\theta_\star) \,|\, \Omega_p, \, \sigma\big(Y_{1:t_p}, \vartheta^{1:\tilde N}_{t_0:t_{p-2}}, \, \theta^{1:N}_{t_0:t_{p-1}}\big)\big) \\ &\geq \mathbb{P}\big(\exists n \in 1:M \text{ s.t. } \vartheta^{N+n}_{t_{p-1}} \in B_{c_\star\tilde\epsilon_p}(\theta_\star) \,|\, \Omega'_p, \, \Omega_p, \, \sigma\big(Y_{1:t_p}, \vartheta^{1:\tilde N}_{t_0:t_{p-2}}, \, \theta^{1:N}_{t_0:t_{p-1}}\big)\big) \\ &= \mathbb{P}\big(\exists n \in 1:M \text{ s.t. } \vartheta^{N+n}_{t_{p-1}} \in B_{c_\star\tilde\epsilon_p}(\theta_\star) \,|\, \Omega_p, \, \sigma\big(Y_{1:t_p}, \vartheta^{1:\tilde N}_{t_0:t_{p-2}}, \, \theta^{1:N}_{t_0:t_{p-1}}\big)\big) \end{aligned} \tag{S.82}$$

showing the first part of the lemma with $\Omega_{p,\tilde\epsilon_p} = \Omega_p$.

To complete the proof we find a lower bound for the probability appearing on the r.h.s. of the equality sign.

Let $c_\nu = \Gamma((\nu+d)/2)/(\Gamma(\nu/2)(\pi\nu)^{d/2})$ and $c' = \|\theta_\star\| \vee \sup_{\mu\in\Theta}\|g(\mu)\|$, with $g$ as in C2. Since, $\mathbb{P}$-almost surely,

$$x^T \Sigma^{-1}_{t_{p-1}} x \leq d\|\Sigma^{-1}_{t_{p-1}}\|\|x\|^2, \quad \forall x \in \mathbb{R}^d,$$

$|\Sigma_{t_{p-1}}| \leq \|\Sigma_{t_{p-1}}\|^d$ and $\sup_{p\geq 0}\|\Sigma_{t_p}\| < +\infty$, we have, $\mathbb{P}$-almost surely,

$$\begin{aligned} \inf_{\{\|\theta\|\leq c', \, \|\theta'\|\leq c'\}} t_\nu\big(\theta; \theta', \Sigma_{t_{p-1}}\big) &\geq c_\nu \, |\Sigma_{t_{p-1}}|^{-\frac{1}{2}}\Big(1 + \nu^{-1}(2c')^2 d\|\Sigma^{-1}_{t_{p-1}}\|\Big)^{-\frac{\nu+d}{2}} \\ &\geq \underline{c}\,\|\Sigma_{t_{p-1}}\|^{-\frac{d}{2}}\|\Sigma^{-1}_{t_{p-1}}\|^{-\frac{\nu+d}{2}} \\ &\geq \underline{c}\,\gamma^\nu_{t_{p-1}} \end{aligned}$$

for a constant $\underline{c} > 0$ and where the last inequality holds under C2.

For $p$ large enough, $\{\vartheta_{t_{p-1}}^{N+1} \in B_{c_\star \tilde{\epsilon}_p}(\theta_\star)\} \subseteq \{\|\vartheta_{t_{p-1}}^{N+1}\| \leq c'\}$ so that, using (S.82) and for $p$ sufficiently large, we have $\mathbb{P}$-almost surely

$$
\begin{aligned}
&\mathbb{P}\big(\bar{\vartheta}_{t_p}^{(2)} \in B_{\tilde{\epsilon}_p}(\theta_\star) \,|\, \Omega_p,\, \sigma\big(Y_{1:t_p}, \vartheta_{t_0:t_{p-2}},\, \theta_{t_0:t_{p-1}}\big)\big) \\
&\qquad \geq \mathbb{P}\big(\exists n \in 1:M \text{ s.t. } \vartheta_{t_{p-1}}^{N+n} \in B_{c_\star \tilde{\epsilon}_p}(\theta_\star) \,|\, \Omega_p,\, \sigma\big(Y_{1:t_p}, \vartheta_{t_0:t_{p-2}}^{1:\tilde{N}},\, \theta_{t_0:t_{p-1}}^{1:N}\big)\big) \\
&\qquad \geq \mathbb{P}\big(\vartheta_{t_{p-1}}^{N+1} \in B_{c_\star \tilde{\epsilon}_p}(\theta_\star) \,|\, \Omega_p,\, \sigma\big(Y_{1:t_p}, \vartheta_{t_0:t_{p-2}}^{1:\tilde{N}},\, \theta_{t_0:t_{p-1}}^{1:N}\big)\big) \\
&\qquad \geq \underline{c}\, \gamma_{t_{p-1}}^{\nu}\, (c_\star \tilde{\epsilon}_p)^d.
\end{aligned}
$$

The proof is complete upon noting that the above computations do not depend on $N$ and $M$. □

# References


Borwein, J. M. and Borwein, P. B. (1987). *Pi and the AGM: A Study in Analytic Number Theory and Computational Complexity.* Wiley, New York.

Kleijn, B. and van der Vaart, A. (2012). The Bernstein-von-Mises theorem under misspecification. *Electronic Journal of Statistics*, 6:354–381.
